# Supplementary material for: Adaptive inference for a semiparametric generalized autoregressive conditional heteroskedasticity model
Source: arXiv:1907.04147 ancillary file (2020-10-02)
Supplement: Supplementary file 1 [file Supplement.pdf]

# SUPPLEMENT TO "ADAPTIVE INFERENCE FOR A SEMIPARAMETRIC GENERALIZED AUTOREGRESSIVE CONDITIONAL HETEROSCEDASTICITY MODEL"

FEIYU JIANG*, DONG LI† AND KE ZHU‡

*Tsinghua University*†* and University of Hong Kong*‡

This supplement provides the additional proofs of the paper.

## APPENDIX B: PROOFS OF LEMMAS AND THEOREMS

PROOF OF LEMMA A.1. See the proof of Lemma 1 in Hafner and Linton (2010). □

PROOF OF LEMMA A.2. (i) By Lemma A.1, $\sup_t |\tau_t - \widehat{\tau}_t| = O(\kappa_T)$. Hence, by Taylor's expansion and Assumption 2.2(ii),

$$\begin{aligned} \widehat{\tau}_t^{-1} &= \tau_t^{-1}\Big(1+\frac{\widehat{\tau}_t-\tau_t}{\tau_t}\Big)^{-1} \\ &= \tau_t^{-1}\Big\{1+\frac{\tau_t-\widehat{\tau}_t}{\tau_t}+O(\kappa_T^2)\Big\} = \tau_t^{-1}+\tau_t^{-2}(\tau_t-\widehat{\tau}_t)+O(\kappa_T^2), \end{aligned} \tag{B.1}$$

where $O(1)$ holds uniformly in $t$. The result (i) follows by noting that $\Delta_t = y_t^2(\widehat{\tau}_t^{-1} - \tau_t^{-1})$.

(ii) Given initial values $\widehat{u}_0 = u_0, ..., \widehat{u}_{1-q} = u_{1-q}, \widehat{g}_0(\theta) = g_0, ..., \widehat{g}_{1-p}(\theta) = g_{1-p}$, we have that for any $\theta \in \Theta$,

$$\begin{aligned} \widetilde{g}_t(\theta) &= \sum_{k=0}^{t-q-1} B^k(1,1)\Big(\omega+\sum_{i=1}^{q}\alpha_i u_{t-k-i}^2\Big)+g_{initial,t}(\theta), \\ \widehat{g}_t(\theta) &= \sum_{k=0}^{t-q-1} B^k(1,1)\Big(\omega+\sum_{i=1}^{q}\alpha_i \widehat{u}_{t-k-i}^2\Big)+g_{initial,t}(\theta), \end{aligned} \tag{B.2}$$

where $B^k(1,1)$ is the $(1,1)$th element of $B^k$, and $g_{initial,t}(\theta) = \sum_{k=1}^{q} B^{t-k}(1,1)\big(\omega + \sum_{i=1}^{q} \alpha_i \widehat{u}_{k-i}^2\big) + B^t(1,1)g_0$. Then, by (B.2) we obtain

$$\widehat{g}_t(\theta) - \widetilde{g}_t(\theta) = \sum_{k=0}^{t-q-1} B^k(1,1)\Big(\sum_{i=1}^{q}\alpha_i\Delta_{t-k-i}\Big) \tag{B.3}$$

and

$$\frac{\widetilde{g}_t(\theta)-\widehat{g}_t(\theta)}{\widehat{g}_t(\theta)} = \frac{-\sum_{k=0}^{t-q-1}B^k(1,1)\big(\sum_{i=1}^{q}\alpha_i\Delta_{t-k-i}\big)}{\sum_{k=0}^{t-1}B^k(1,1)\big(\omega+\sum_{i=1}^{q}\alpha_i\widehat{u}_{t-k-i}^2\big)+B^t(1,1)g_0}. \tag{B.4}$$

Next, by (B.1) and the result (i), we have

$$\frac{|\Delta_t|}{\widehat{u}_t^2} = \frac{|\Delta_t|}{u_t^2}\frac{\widehat{\tau}_t}{\tau_t} = \frac{|\Delta_t|}{u_t^2}\Big\{1 + \frac{\tau_t - \widehat{\tau}_t}{\tau_t} + O(\kappa_T^2)\Big\}$$
$$= \Big|\frac{\tau_t - \widehat{\tau}_t}{\tau_t} + O(\kappa_T^2)\Big|\Big\{1 + \frac{\tau_t - \widehat{\tau}_t}{\tau_t} + O(\kappa_T^2)\Big\} = O(\kappa_T),$$

where the last equality holds since $\sup_t |\tau_t - \widehat{\tau}_t| = O(\kappa_T)$ by Lemma A.1. Thus, by (B.4) it follows that

$$\sup_t \frac{|\widetilde{g}_t(\theta) - \widehat{g}_t(\theta)|}{\widehat{g}_t(\theta)} \leq O(\kappa_T). \tag{B.5}$$

Now, the result (ii) follows by noting that $\widetilde{S}_t(\theta) = \frac{\widetilde{g}_t(\theta)-\widehat{g}_t(\theta)}{\widetilde{g}_t(\theta)\widehat{g}_t(\theta)}$ and $\sup_{\theta\in\Theta}\frac{1}{\widetilde{g}_t(\theta)} \leq \sup_{\theta\in\Theta}\frac{1}{\omega} < \infty$ by the compactness of $\Theta$. □

Proof of Lemma A.3. For simplicity, we only show the the proof of (ii), since the proofs of (i) and (iii) are similar. By a direct calculation, we have

$$\frac{\partial\widetilde{g}_t(\theta)}{\partial\alpha_i} = \sum_{k=0}^{t-q-1} B^k(1,1)(u_{t-k-i}^2 - 1) + \sum_{k=1}^{q} B^{t-k}(1,1)(\widehat{u}_{k-i}^2 - 1) + B^t(1,1)\frac{\partial\widehat{g}_0(\theta)}{\partial\alpha_i},$$
$$\frac{\partial\widetilde{g}_t(\theta)}{\partial\beta_j} = \sum_{k=1}^{t-q-1}\Big(\sum_{i=1}^{k} B^{i-1}B^{(j)}B^{k-i}\Big)(1,1)\Big(\omega + \sum_{i=1}^{q}\alpha_i u_{t-k-i}^2\Big) - \sum_{k=0}^{t-1} B^k(1,1)$$
$$+ \sum_{k=1}^{q}\Big(\sum_{i=1}^{t-k} B^{i-1}B^{(j)}B^{t-k-i}\Big)(1,1)\Big(\omega + \sum_{i=1}^{q}\alpha_i\widehat{u}_{k-i}^2\Big).$$

Similarly, we can write down the expressions of $\frac{\partial\widehat{g}_t(\theta)}{\partial\alpha_i}$ and $\frac{\partial\widehat{g}_t(\theta)}{\partial\beta_j}$. Then, we can show

$$\frac{\partial\widetilde{g}_t(\theta)}{\partial\alpha_i} - \frac{\partial\widehat{g}_t(\theta)}{\partial\alpha_i} = -\sum_{k=0}^{t-q-1} B^k(1,1)\Delta_{k-i},$$
$$\frac{\partial\widetilde{g}_t(\theta)}{\partial\beta_j} - \frac{\partial\widehat{g}_t(\theta)}{\partial\beta_j} = -\sum_{k=1}^{t-q-1}\Big(\sum_{i=1}^{k} B^{i-1}B^{(j)}B^{k-i}\Big)(1,1)\Big(\sum_{i=1}^{q}\alpha_i\Delta_{t-k-i}\Big).$$

By Lemma A.1 and Lemma A.2(i), we have

$$|\Delta_t| \leq C\kappa_T u_t^2. \tag{B.6}$$

Now, the result (ii) holds by Minkowski's inequality and the fact that $\sup_{\theta\in\Theta}\rho(B) < 1$. □

Proof of Lemma A.4. The proofs of (i)–(iii) are similar to those of Theorems 2.1–2.2 in Francq and Zakoïan (2004), hence they are omitted. □

Proof of Lemma A.5. Using the following recursive representations:

$$\frac{\partial g_t(\theta)}{\partial\alpha_i} = -1 + u_{t-i}^2 + \sum_{k=1}^{p}\beta_k\frac{\partial g_{t-k}(\theta)}{\partial\alpha_i} \quad \text{and} \quad \frac{\partial g_t(\theta)}{\partial\beta_j} = -1 + \sum_{k=1}^{p}\beta_k\frac{\partial g_{t-k}(\theta)}{\partial\beta_j} + g_{t-j}(\theta),$$

the result follows by using the proof of Proposition 12 in Carrasco and Chen (2002) with some minor modifications. □

Proof of Theorem 2.1. Recall $z_t = u_t^2 - 1$. By Lemma A.5, $z_t$ is $\beta$-mixing, and then the result follows directly by Lemma A.1 and the central limit theorem for mixing process (see Hall and Heyde (1980)). □

Proof of Theorem 2.2(i). By Theorem 4.1.1 in Amemiya (1985), it suffices to show the following intermediate results:

(1) $E|l_t(\theta_0)| < \infty$ and $\theta_0$ is the unique minimizer of $El_t(\theta)$;

(2) $\sup_{\theta\in\Theta}\left|T^{-1}L_T(\theta) - El_t(\theta)\right| = o_p(1)$ and $\sup_{\theta\in\Theta}\left|T^{-1}\widetilde{L}_T(\theta) - T^{-1}L_T(\theta)\right| = o_p(1)$;

(3) $\sup_{\theta\in\Theta}\left|T^{-1}\widehat{L}_T(\theta) - T^{-1}\widetilde{L}_T(\theta)\right| = o_p(1)$.

Using Lemma A.4, the proofs of results (1)–(2) are similar to that of Theorem 2.1 in Francq and Zakoïan (2004). Below, it suffices to prove the result (3). Note that

$$\begin{aligned}
&\sup_{\theta\in\Theta}\left|T^{-1}\widehat{L}_T(\theta) - T^{-1}\widetilde{L}_T(\theta)\right| \\
\le& T^{-1}\sum_{t=1}^{T}\sup_{\theta\in\Theta}\left\{\left|\frac{\widehat{u}_t^2}{\widetilde{g}_t(\theta)} - \frac{u_t^2}{\widetilde{g}_t(\theta)}\right| + \left|\log\left(1 + \frac{\widehat{g}_t(\theta) - \widetilde{g}_t(\theta)}{\widetilde{g}_t(\theta)}\right)\right|\right\} \\
\le& T^{-1}\sum_{t=1}^{T}\sup_{\theta\in\Theta}\left\{\left|\frac{\Delta_t}{\widetilde{g}_t(\theta)}\right| + \left|\widetilde{S}_t(\theta)u_t^2\right| + \left|\widetilde{S}_t(\theta)\Delta_t\right|\right\} \\
&+ T^{-1}\sum_{t=1}^{T}\sup_{\theta\in\Theta}\left\{\left|\log\left(1 + \frac{\widehat{g}_t(\theta) - \widetilde{g}_t(\theta)}{\widetilde{g}_t(\theta)}\right)\right|\right\}.
\end{aligned} \tag{B.7}$$

The first term in (B.7) is $o_p(1)$ by Lemma A.2(ii), (B.6) and Assumption 2.4. Moreover, the second term in (B.7) is $o_p(1)$ by using the inequality $\log(x) \le x - 1$ and (B.5). Hence, the result (3) holds. □

Proof of Lemma A.9. First, observe that

$$\begin{aligned}
\left|\tau_t^{-1}(\widehat{\tau}_t - \tau_t) - \tau_{t-i}^{-1}(\widehat{\tau}_{t-i} - \tau_{t-i})\right| &= \left|\tau_t^{-1}\widehat{\tau}_t - \tau_{t-i}^{-1}\widehat{\tau}_{t-i}\right| \\
&\le \left|\tau_t^{-1}(\widehat{\tau}_t - \widehat{\tau}_{t-i})\right| + \left|(\tau_t^{-1} - \tau_{t-i}^{-1})\widehat{\tau}_{t-i}\right| \\
&:= I_{1ti} + I_{2ti}.
\end{aligned}$$

Next, we have that for any $0 < s - s' < m_T$,

$$|\widehat{\tau}_s - \widehat{\tau}_{s'}| = \frac{1}{Th}\left|\sum_{t=s'-[Th]}^{s+[Th]}\left\{K\Big(\frac{s-t}{Th}\Big) - K\Big(\frac{s'-t}{Th}\Big)\right\}y_t^2\right|$$

$$
\begin{aligned}
&\le \frac{1}{Th}\sum_{t=s'-[Th]}^{s'+m_T+[Th]}\Big|K\Big(\frac{s-t}{Th}\Big)-K\Big(\frac{s'-t}{Th}\Big)\Big|y_t^2\\
&\le C\frac{m_T}{T^2h^2}\sum_{t=s'-[Th]}^{s'+m_T+[Th]}\overline{\tau}u_t^2\\
&\le C\frac{m_T(m_T+2Th)}{T^2h^2}(Eu_t^2+1)=o\Big(\frac{1}{\sqrt{T}}\Big),
\end{aligned}
$$

where the first inequality holds since $K(x)=0$ for $|x|>1$, the second inequality holds by Assumption 2.2(ii) and the fact that $\big|K(\frac{s-t}{Th})-K(\frac{s'-t}{Th})\big|\le\frac{C|s-s'|}{Th}$ by Lipschitz condition of $K(\cdot)$, and the third inequality holds by the ergodic theorem. Since $|\tau_t^{-1}|\le\underline{\tau}^{-1}$ by Assumption 2.2(ii), it follows that uniformly in $t$ and $i$, $|I_{1ti}|\le o\big(\frac{1}{\sqrt{T}}\big)$ a.s. Similarly, we have that uniformly in $t$ and $i$, $|I_{2ti}|=o\big(\frac{1}{\sqrt{T}}\big)$ by noting that $\tau_t^{-1}=\tau_{t-i}^{-1}+o\big(\frac{1}{\sqrt{T}}\big)$ for $i\le m_T$, and $\sup_t|\widehat{\tau}_t|<\infty$ a.s. by Lemma A.1. Now, the result follows. □

Proof of Lemma A.10. For simplicity, we only show that $U_3=o_p(1)$, since the proof for $U_2$ is similar.

First, by (B.2) and Lemma A.4, it is not hard to show

$$
\begin{aligned}
U_3=&\frac{1}{\sqrt{T}}\sum_{t=1}^{T}(1-g_t^{-1}u_t^2)\widetilde{S}_t\frac{\partial g_t}{\partial\theta_m}+o_p(1)\\
=&\frac{1}{\sqrt{T}}\sum_{t=1}^{T}(1-\eta_t^2)g_t^{-2}(\widetilde{g}_t-\widehat{g}_t)\frac{\partial g_t}{\partial\theta_m}+o_p(1)\\
=&\frac{1}{\sqrt{T}}\sum_{t=q+1}^{T}(\eta_t^2-1)g_t^{-2}\frac{\partial g_t}{\partial\theta_m}\Big\{\sum_{k=0}^{t-q-1}B_0^k(1,1)\Big(\sum_{i=1}^{q}\alpha_{i0}\Delta_{t-k-i}\Big)\Big\}+o_p(1)\\
:=&\sum_{i=1}^{q}\alpha_{i0}U_{3i}+o_p(1),
\end{aligned}
$$

where

$$
U_{3i}=\frac{1}{\sqrt{T}}\sum_{k=0}^{T-q-1}B_0^k(1,1)\sum_{t=k+q+1}^{T}(\eta_t^2-1)g_t^{-2}\frac{\partial g_t}{\partial\theta_m}\Delta_{t-k-i}.
$$

Next, by Lemma A.2 and the fact that $O(\kappa_T^2)=o(T^{-1/2})$, we have

$$
\Delta_{t-k-i}=\tau_{t-k-i}^{-1}(\tau_{t-k-i}-\widehat{\tau}_{t-k-i})u_{t-k-i}^2+o_p(T^{-1/2}).
$$

Let $m_T$ be defined as in (A.10). Then, by Lemma A.9, we can show that for $1\le k\le m_T$,

$$
\Delta_{t-k-i}=\tau_t^{-1}(\tau_t-\hat{\tau}_t)u_{t-k-i}^2+o_p(T^{-1/2}). \tag{B.8}
$$

Furthermore, let $\phi_{tki} = (\eta_t^2 - 1)g_t^{-2}\frac{\partial g_t}{\partial \theta_m}u_{t-k-i}^2$. By (B.8), $U_{3i} = U_{3i1} + U_{3i2} + o_p(1)$, where

$$U_{3i1} = \frac{1}{\sqrt{T}}\sum_{k=0}^{m_T} B_0^k(1,1)\sum_{t=k+q+1}^{T}\phi_{tki}\tau_t^{-1}(\tau_t - \widehat{\tau}_t),$$
$$U_{3i2} = \frac{1}{\sqrt{T}}\sum_{k=m_T+1}^{T-q-1} B_0^k(1,1)\sum_{t=k+q+1}^{T}\phi_{tki}\tau_{t-k-i}^{-1}(\tau_{t-k-i} - \widehat{\tau}_{t-k-i}).$$

Since $E|\phi_{tki}| < \infty$ by Assumption 2.6, $\sup_t |\tau_t^{-1}(\tau_t - \widehat{\tau}_t)|$ by Lemma A.1, and $\rho_{B_0} < 1$, it follows that $U_{3i2} = o_p(1)$ due to $TB_0^{m_T}(1,1) \to 0$. Hence, we obtain

$$\begin{aligned}U_3 =& \frac{1}{\sqrt{T}}\sum_{k=0}^{m_T} B_0^k(1,1)\sum_{t=k+q+1}^{T}(\eta_t^2 - 1)g_t^{-2}\frac{\partial g_t}{\partial \theta_m}\tau_t^{-1}(\tau_t - \widehat{\tau}_t)\Big(\sum_{i=1}^{q}\alpha_{i0}u_{t-k-i}^2\Big) + o_p(1)\\ =& \frac{1}{\sqrt{T}}\sum_{t=q+1}^{T}(\eta_t^2 - 1)g_t^{-2}\frac{\partial g_t}{\partial \theta_m}\tau_t^{-1}(\tau_t - \widehat{\tau}_t)\sum_{k=0}^{\min\{t-q-1, m_T\}} B_0^k(1,1)\Big(\sum_{i=1}^{q}\alpha_{i0}u_{t-k-i}^2\Big) + o_p(1),\end{aligned}$$

or equivalently,

$$\begin{aligned}U_3 =& \frac{1}{\sqrt{T}}\sum_{t=q+1}^{T}\Big\{(\eta_t^2 - 1)g_t^{-2}\frac{\partial g_t}{\partial \theta_m}\tau_t^{-1}(\tau_t - \widehat{\tau}_t)\sum_{k=0}^{\infty} B_0^k(1,1)\Big(\sum_{i=1}^{q}\alpha_{i0}u_{t-k-i}^2\Big)\\ &- (\eta_t^2 - 1)g_t^{-2}\frac{\partial g_t}{\partial \theta_m}\tau_t^{-1}(\tau_t - \widehat{\tau}_t)\sum_{k=\max\{t-q, m_T+1\}}^{\infty} B_0^k(1,1)\Big(\sum_{i=1}^{q}\alpha_{i0}u_{t-k-i}^2\Big)\Big\}\\ &+ o_p(1). \qquad \text{(B.9)}\end{aligned}$$

Again, by using $E|\phi_{tki}| < \infty$, Lemma A.1 and Markov's inequality, we have

$$\begin{aligned}&E\Big|\frac{1}{\sqrt{T}}\sum_{t=q+1}^{T}(\eta_t^2 - 1)g_t^{-2}\frac{\partial g_t}{\partial \theta_m}\tau_t^{-1}(\tau_t - \widehat{\tau}_t)\sum_{k=\max\{t-q, m_T+1\}}^{\infty} B_0^k(1,1)\Big(\sum_{i=1}^{q}\alpha_{i0}u_{t-k-i}^2\Big)\Big|\\ \le& \sup_t |\tau_t^{-1}(\tau_t - \widehat{\tau}_t)|\frac{1}{\sqrt{T}}\sum_{t=q+1}^{T}\sum_{k=\max\{t-q, m_T+1\}}^{\infty} B_0^k(1,1)\sum_{i=1}^{q}\alpha_{i0}E|\phi_{tki}|\\ =& O(\kappa_T)\frac{1}{\sqrt{T}}\Big(\sum_{t=q+1}^{m_T}\rho_{B_0}^t + \sum_{t=m_T}^{T}\rho_{B_0}^{m_T}\Big) = o(1).\end{aligned}$$

Together with (B.9) and the fact that $g_t(\theta_0) = \sum_{k=0}^{\infty} B_0^k(1,1)(\omega_0 + \sum_{i=1}^{q}\alpha_{i0}u_{t-k-i}^2)$, it follows that

$$\begin{aligned}U_3 =& \frac{1}{\sqrt{T}}\sum_{t=q+1}^{T}(\eta_t^2 - 1)g_t^{-2}\frac{\partial g_t}{\partial \theta_m}\tau_t^{-1}(\tau_t - \widehat{\tau}_t)\sum_{k=0}^{\infty} B_0^k(1,1)\Big(\sum_{i=1}^{q}\alpha_{i0}u_{t-k-i}^2\Big) + o_p(1)\\ =& \frac{1}{\sqrt{T}}\sum_{t=q+1}^{T}(\eta_t^2 - 1)g_t^{-2}\frac{\partial g_t}{\partial \theta_m}\tau_t^{-1}(\tau_t - \widehat{\tau}_t)\Big(g_t - \sum_{k=0}^{\infty} B_0^k(1,1)\omega_0\Big) + o_p(1).\end{aligned}$$

Note that

$$1 = Eg_t(\theta_0) = \sum_{k=0}^{\infty} B_0^k(1,1)\Big(\omega_0 + \sum_{i=1}^{q}\alpha_{i0}\Big) = \sum_{k=0}^{\infty} B_0^k(1,1)\Big(1 - \sum_{j=1}^{p}\beta_{j0}\Big),$$

which gives us

$$\sum_{k=0}^{\infty} B_0^k(1,1) = 1/\gamma_0. \tag{B.10}$$

Using Lemma A.1, it follows that

$$U_3 = -\frac{1}{\sqrt{T}}\sum_{t=q+1}^{T}(\eta_t^2-1)g_t^{-2}\frac{\partial g_t}{\partial\theta_m}\Big(g_t - \frac{\omega_0}{\gamma_0}\Big)\Big\{\frac{1}{Th}\sum_{s=1}^{T}K\Big(\frac{t-s}{Th}\Big)z_s\Big\} + o_p(1) := U_3^* + o_p(1).$$

Third, we show

$$\mathrm{Var}(U_3^*) = o(1). \tag{B.11}$$

Recall $z_t = u_t^2 - 1$. To prove (B.11) by Proposition A.1 with $a_t = z_t$, $c_t = (u_t^2, g_t, \frac{\partial g_t}{\partial\theta'})'$ and $b_t = (\eta_t^2-1)g_t^{-2}\frac{\partial g_t}{\partial\theta_m}(g_t - \frac{\omega_0}{\gamma_0})$, it remains to verify Conditions 1–4 in this proposition. By Assumptions 2.6 and 2.7(ii), $\xi := \frac{2}{4(1+\delta_0)} + \frac{2}{4+4/\delta_0+\delta_1} < \frac{1}{2}$. Hence, by letting $\delta = \frac{1}{4\xi} - \frac{1}{2} > 0$, $\iota_1 = \frac{2(1+\delta_0)}{1+2\delta}$ and $\iota_2 = \frac{4+4/\delta_0+\delta_1}{2(1+2\delta)}$, we have that $E|a_t|^{\iota_1(1+2\delta)} = E|u_t^2-1|^{2(1+\delta_0)}$ and $E|b_t|^{\iota_2(1+2\delta)} = E|b_t|^{2+2/\delta_0+\delta_1/2}$. Using Assumption 2.7(ii) and the fact that $E\big|g_t^{-1}\frac{\partial g_t}{\partial\theta_m}\big|^d < \infty$ for any integer $d$ (see (4.29) in Francq and Zakoïan (2004)), we can show that $E|b_t|^{4+4/\delta_0+\delta_1} \le O(\kappa_T)E(\eta_t^2-1)^{2+2/\delta_0+\delta_1/2}E\big|g_t^{-1}\frac{\partial g_t}{\partial\theta_m}\big|^{2+2/\delta_0+\delta_1/2} < \infty$, and hence Condition (1) holds. Next, Condition (2) holds by Lemma A.5, and Conditions (3)–(4) hold by Assumption 2.8 and (A.10). Now, we can claim that $U_3^* = o_p(1)$ by Chebyshev's inequality, and the result thus follows. □

Proof of Lemma A.11. First, by (B.3), Lemma A.4 and Lemma A.10, we have

$$\begin{aligned} U_5 =& U_3 - \frac{1}{\sqrt{T}}\sum_{t=1}^{T}\widetilde{S}_t\frac{\partial\widetilde{g}_t}{\partial\theta_m} \\ =& \frac{1}{\sqrt{T}}\sum_{t=1}^{T}g_t^{-2}(\widehat{g}_t - \widetilde{g}_t)\frac{\partial g_t}{\partial\theta_m} + o_p(1) \\ =& \frac{1}{\sqrt{T}}\sum_{k=0}^{T-q-1}B_0^k(1,1)\sum_{i=1}^{q}\alpha_{i0}\sum_{t=k+q+1}^{T}g_t^{-2}\frac{\partial g_t}{\partial\theta_m}\Delta_{t-k-i} + o_p(1). \end{aligned}$$

By Lemma A.1 and similar arguments used in Lemma A.10, we have

$$U_5 = \frac{1}{\sqrt{T}}\sum_{t=q+1}^{T}g_t^{-2}\frac{\partial g_t}{\partial\theta_m}\tau_t^{-1}(\tau_t - \widehat{\tau}_t)\sum_{k=0}^{\infty}B_0^k(1,1)\sum_{i=1}^{q}\alpha_{i0}u_{t-k-i}^2 + o_p(1).$$

Using the fact that $g_t(\theta_0) = \sum_{k=0}^{\infty} B_0^k(1,1)(\omega_0 + \sum_{i=1}^{q} \alpha_{i0} u_{t-k-i}^2)$ and (B.10), we have

$$U_5 = \frac{1}{\sqrt{T}} \sum_{t=q+1}^{T} g_t^{-2} \frac{\partial g_t}{\partial \theta_m} \tau_t^{-1}(\tau_t - \widehat{\tau}_t)\Big(g_t - \frac{\omega_0}{\gamma_0}\Big) + o_p(1) := U_5^* + o_p(1). \tag{B.12}$$

We decompose $U_5^* = U_{51}^* + U_{52}^*$, where

$$\begin{aligned} U_{51}^* =& \frac{1}{\sqrt{T}} \sum_{t=q+1}^{T} E\Big\{g_t^{-2} \frac{\partial g_t}{\partial \theta_m}\Big(g_t - \frac{\omega_0}{\gamma_0}\Big)\Big\}\tau_t^{-1}(\tau_t - \widehat{\tau}_t), \\ U_{52}^* =& \frac{1}{\sqrt{T}} \sum_{t=q+1}^{T} \Big\{\Big(g_t^{-2} \frac{\partial g_t}{\partial \theta_m}\Big(g_t - \frac{\omega_0}{\gamma_0}\Big)\Big) - E\Big(g_t^{-2} \frac{\partial g_t}{\partial \theta_m}\Big(g_t - \frac{\omega_0}{\gamma_0}\Big)\Big)\Big\}\tau_t^{-1}(\tau_t - \widehat{\tau}_t). \end{aligned}$$

Letting $a_t = z_t$, $b_t = \big\{\big(g_t^{-2} \frac{\partial g_t}{\partial \theta_m}(g_t - \frac{\omega_0}{\gamma_0})\big) - M_m\big\}$, and $c_t = (u_t^2, g_t, \frac{\partial g_t}{\partial \theta'})'$, it is easy to see that Conditions 1-4 in Proposition A.1 hold. Hence,

$$U_{52}^* = o_p(1). \tag{B.13}$$

Next, since $\frac{1}{Th}\sum_{t=q+1}^{T} K\big(\frac{s-t}{Th}\big) = 1 + O\big(\frac{1}{Th}\big)$ uniformly in $s$, we can obtain

$$\begin{aligned} U_{51}^* =& -\frac{1}{\sqrt{T}} \sum_{t=q+1}^{T} M_m \frac{1}{Th} \sum_{s=1}^{T} K\Big(\frac{t-s}{Th}\Big) z_s = -\frac{1}{Th} \sum_{t=q+1}^{T} K\Big(\frac{t-s}{Th}\Big) M_m \frac{1}{\sqrt{T}} \sum_{s=1}^{T} z_s \\ =& -\frac{1}{\sqrt{T}} \sum_{s=1}^{T} M_m z_s + o_p(1). \end{aligned}$$

Finally, the result follows by (B.12)–(B.13). □

Proof of Lemma A.12. Using Lemmas A.2 and A.4, we can show

$$U_9 = \frac{1}{\sqrt{T}} \sum_{t=1}^{T} \tau_t^{-1} \eta_t^2 g_t^{-1} \frac{\partial g_t}{\partial \theta_m}(\widehat{\tau}_t - \tau_t) + o_p(1).$$

Next, by Lemma A.1, we have

$$U_9 = \frac{1}{\sqrt{T}} \sum_{s=1}^{T} \frac{z_s}{Th} \sum_{t=1}^{T} K\Big(\frac{t-s}{Th}\Big) g_t^{-1} \frac{\partial g_t}{\partial \theta_m} + o_p(1) := U_{91} + U_{92} + o_p(1),$$

where

$$\begin{aligned} U_{91} =& \frac{1}{\sqrt{T}} \sum_{t=1}^{T} E\Big(\frac{1}{g_t}\frac{\partial g_t}{\partial \theta_m}\Big) \frac{1}{Th} \sum_{s=1}^{T} K\Big(\frac{t-s}{Th}\Big) z_s, \\ U_{92} =& \frac{1}{\sqrt{T}} \sum_{t=1}^{T} \Big\{\frac{1}{g_t}\frac{\partial g_t}{\partial \theta_m} - E\Big(\frac{1}{g_t}\frac{\partial g_t}{\partial \theta_m}\Big)\Big\} \frac{1}{Th} \sum_{s=1}^{T} K\Big(\frac{t-s}{Th}\Big) z_s. \end{aligned}$$

By using the fact that $\frac{1}{Th}\sum_{t=1}^{T} K\big(\frac{t-s}{Th}\big) = 1 + O\big(\frac{1}{Th}\big)$ for any $s$, it is not hard to see

$$U_{91} = \frac{1}{\sqrt{T}} E\Big(\frac{1}{g_t}\frac{\partial g_t}{\partial \theta_m}\Big) \sum_{s=1}^{T} z_s + o_p(1).$$

Since $U_{92} = o_p(1)$ by the similar argument as for (B.13), the result follows. □

Proof of Theorem 3.1. The Lagrangian can be formulated as

$$\mathcal{L}(\theta, \lambda) = \widehat{L}_T(\theta) - \lambda'(R\theta - r),$$

and $(\widehat{\theta}_{T|0}, \widehat{\lambda}) = \arg\inf_{\theta,\lambda} \mathcal{L}(\theta, \lambda)$. First, the first order condition gives us

$$R'\widehat{\lambda} = \frac{\partial \widehat{L}_T(\widehat{\theta}_{T|0})}{\partial \theta} \quad \text{and} \quad R\widehat{\theta}_{T|0} = r. \tag{B.14}$$

By similar arguments as for Theorem 2.2 and Taylor's expansion, we have

$$\frac{R'\widehat{\lambda}}{\sqrt{T}} = \frac{1}{\sqrt{T}}\frac{\partial \widehat{L}_T(\widehat{\theta}_{T|0})}{\partial \theta} = \frac{1}{\sqrt{T}}\frac{\partial \widehat{L}_T(\theta_0)}{\partial \theta} + J_1\sqrt{T}(\widehat{\theta}_{T|0} - \theta_0) + o_p(1).$$

Multiplying both sides of the preceding equation by $RJ_1^{-1}$, we can obtain

$$\frac{RJ_1^{-1}R'\widehat{\lambda}}{\sqrt{T}} = \frac{RJ_1^{-1}}{\sqrt{T}}\frac{\partial \widehat{L}_T(\theta_0)}{\partial \theta} + R\sqrt{T}(\widehat{\theta}_{T|0} - \theta_0) + o_p(1).$$

Under $\mathbb{H}_0$ and (B.14), $R\sqrt{T}(\widehat{\theta}_{T|0} - \theta_0) = 0$. Hence, using the fact that $\frac{1}{\sqrt{T}}\frac{\partial \widehat{L}_T(\theta_0)}{\partial \theta} \to_{\mathcal{L}} N(0, J_1\Sigma J_1)$, it follows that

$$\frac{\widehat{\lambda}}{\sqrt{T}} = (RJ_1^{-1}R')^{-1}\frac{RJ_1^{-1}}{\sqrt{T}}\frac{\partial \widehat{L}_T(\theta_0)}{\partial \theta} + o_p(1) \to_{\mathcal{L}} N(0, (RJ_1^{-1}R')^{-1}(R\Sigma R')(RJ_1^{-1}R')^{-1}).$$

Now, the result follows directly by (B.14). □

Proof of Lemma A.13. Decompose $R_2 = \sum_{i=1}^{4} R_{2i}$, where

$$R_{21} = \frac{1}{\sqrt{T}} \sum_{t=k+1}^{T} \Big\{\frac{\widehat{u}_t^2}{\widehat{g}_t(\widehat{\theta}_T)} - \frac{u_t^2}{g_t(\widehat{\theta}_T)}\Big\}\Big\{\frac{u_{t-k}^2}{g_{t-k}(\widehat{\theta}_T)} - \frac{u_{t-k}^2}{g_{t-k}(\theta_0)}\Big\},$$

$$R_{22} = \frac{1}{\sqrt{T}} \sum_{t=k+1}^{T} \Big\{\frac{u_t^2}{g_t(\widehat{\theta}_T)} - \frac{u_t^2}{g_t(\theta_0)}\Big\}\Big\{\frac{\widehat{u}_{t-k}^2}{\widehat{g}_{t-k}(\widehat{\theta}_T)} - \frac{u_{t-k}^2}{g_{t-k}(\widehat{\theta}_T)}\Big\},$$

$$R_{23} = \frac{1}{\sqrt{T}} \sum_{t=k+1}^{T} \Big\{\frac{u_t^2}{g_t(\widehat{\theta}_T)} - \frac{u_t^2}{g_t(\theta_0)}\Big\}\Big\{\frac{u_{t-k}^2}{g_{t-k}(\widehat{\theta}_T)} - \frac{u_{t-k}^2}{g_{t-k}(\theta_0)}\Big\},$$

$$R_{24} = \frac{1}{\sqrt{T}} \sum_{t=k+1}^{T} \Big\{\frac{\widehat{u}_t^2}{\widehat{g}_t(\widehat{\theta}_T)} - \frac{u_t^2}{g_t(\widehat{\theta}_T)}\Big\}\Big\{\frac{\widehat{u}_{t-k}^2}{\widehat{g}_{t-k}(\widehat{\theta}_T)} - \frac{u_{t-k}^2}{g_{t-k}(\widehat{\theta}_T)}\Big\}.$$

The result follows by the following quantities:

(i) $R_{21} = o_p(1)$; (ii) $R_{22} = o_p(1)$; (iii) $R_{23} = o_p(1)$; (iv) $R_{24} = o_p(1)$.

(i) Let $S_t(\widehat{\theta}_T) = \frac{1}{\widehat{g}_t(\widehat{\theta}_T)} - \frac{1}{g_t(\widehat{\theta}_T)}$. Then, we can decompose $R_{21} = \sum_{i=1}^3 R_{21i}$, where

$$\begin{aligned}
R_{211} =& \frac{1}{\sqrt{T}} \sum_{t=k+1}^{T} u_t^2 S_t(\widehat{\theta}_T) \Big\{ \frac{u_{t-k}^2}{g_{t-k}(\widehat{\theta}_T)} - \frac{u_{t-k}^2}{g_{t-k}(\theta_0)} \Big\}, \\
R_{212} =& \frac{1}{\sqrt{T}} \sum_{t=k+1}^{T} \Delta_t S_t(\widehat{\theta}_T) \Big\{ \frac{u_{t-k}^2}{g_{t-k}(\widehat{\theta}_T)} - \frac{u_{t-k}^2}{g_{t-k}(\theta_0)} \Big\}, \\
R_{213} =& \frac{1}{\sqrt{T}} \sum_{t=k+1}^{T} \frac{\Delta_t}{g_t(\widehat{\theta}_T)} \Big\{ \frac{u_{t-k}^2}{g_{t-k}(\widehat{\theta}_T)} - \frac{u_{t-k}^2}{g_{t-k}(\theta_0)} \Big\}.
\end{aligned}$$

By Taylor's expansion, we have that for some $\theta^*$ lies between $\widehat{\theta}_T$ and $\theta_0$,

$$\begin{aligned}
R_{211} =& \frac{1}{T} \sum_{t=k+1}^{T} u_t^2 S_t(\widehat{\theta}_T) \frac{u_{t-k}^2}{g_{t-k}^2(\theta^*)} \frac{\partial g_{t-k}(\theta^*)}{\partial \theta} \sqrt{T}(\widehat{\theta}_T - \theta_0) \\
=& \sqrt{T}(\widehat{\theta}_T - \theta_0) \frac{1}{T} \sum_{t=k+1}^{T} \frac{u_t^2}{g_t(\widehat{\theta}_T)} \frac{g_t(\widehat{\theta}_T) - \widehat{g}_t(\widehat{\theta}_T)}{\widehat{g}_t(\widehat{\theta}_T)} \frac{u_{t-k}^2}{g_{t-k}^2(\theta^*)} \frac{\partial g_{t-k}(\theta^*)}{\partial \theta}.
\end{aligned}$$

By (B.4) and Lemma A.4, we have

$$\begin{aligned}
\sup_{\theta\in\Theta} \Big\| \frac{g_t(\theta) - \widehat{g}_t(\theta)}{\widehat{g}_t(\theta)} \Big\|_4 \leq& \sup_{\theta\in\Theta} \Big\| \frac{g_t(\theta) - \widetilde{g}_t(\theta)}{\widehat{g}_t(\theta)} \Big\|_4 + \sup_{\theta\in\Theta} \Big\| \frac{\widetilde{g}_t(\theta) - \widehat{g}_t(\theta)}{\widehat{g}_t(\theta)} \Big\|_4 \\
\leq& C(\kappa_T + \rho^t), \qquad \text{(B.15)}
\end{aligned}$$

and hence,

$$\begin{aligned}
& E \Big\| \frac{1}{T} \sum_{t=k+1}^{T} \frac{u_t^2}{g_t(\widehat{\theta}_T)} \frac{g_t(\widehat{\theta}_T) - \widehat{g}_t(\widehat{\theta}_T)}{\widehat{g}_t(\widehat{\theta}_T)} \frac{u_{t-k}^2}{g_{t-k}^2(\theta^*)} \frac{\partial g_{t-k}(\theta^*)}{\partial \theta} \Big\| \\
\leq& \frac{1}{T} \sum_{t=k+1}^{T} E \Big\| \frac{u_t^2}{g_t(\widehat{\theta}_T)} \Big\| \Big\| \frac{g_t(\widehat{\theta}_T) - \widehat{g}_t(\widehat{\theta}_T)}{\widehat{g}_t(\widehat{\theta}_T)} \Big\| \Big\| \frac{u_{t-k}^2}{g_{t-k}(\theta^*)} \Big\| \Big\| \frac{1}{g_{t-k}(\theta^*)} \frac{\partial g_{t-k}(\theta^*)}{\partial \theta} \Big\| \\
\leq& \frac{1}{T} \sum_{t=k+1}^{T} C(\kappa_T + \rho^t) \Big\| \frac{u_t^2}{g_t(\widehat{\theta}_T)} \Big\|_4 \Big\| \frac{u_{t-k}^2}{g_{t-k}(\theta^*)} \Big\|_4 \Big\| \frac{1}{g_{t-k}(\theta^*)} \frac{\partial g_{t-k}(\theta^*)}{\partial \theta} \Big\|_4 = o(1),
\end{aligned}$$

where the first inequality holds by triangular inequality, the second inequality holds by (B.15) and Hölder's inequality, and the last equality holds by Assumption 2.6. Since $\sqrt{T}(\widehat{\theta}_T - \theta_0) = O_p(1)$, it follows that $R_{211} = o_p(1)$ by using Markov's inequality. Similarly, we can show that $R_{212} = o_p(1)$ and $R_{213} = o_p(1)$ by (B.6).

(ii) It follows by similar arguments as for part (i).

(iii) By Taylor's expansion, it is not hard to show that $R_{23} = o_p(1)$.

(iv) We decompose $R_{24}$ as follows:

$$
\begin{aligned}
R_{24} =&\frac{1}{\sqrt{T}}\sum_{t=k+1}^{T}\Big\{(u_t^2+\Delta_t)S_t(\widehat{\theta}_T)+\frac{\Delta_t}{g_t(\widehat{\theta}_T)}\Big\}\Big\{(u_{t-k}^2+\Delta_{t-k})S_{t-k}(\widehat{\theta}_T)+\frac{\Delta_{t-k}}{g_{t-k}(\widehat{\theta}_T)}\Big\}\\
=&\frac{1}{\sqrt{T}}\sum_{t=k+1}^{T}(u_t^2+\Delta_t)S_t(\widehat{\theta}_T)(u_{t-k}^2+\Delta_{t-k})S_{t-k}(\widehat{\theta}_T)+\frac{1}{\sqrt{T}}\sum_{t=k+1}^{T}\frac{\Delta_t}{g_t(\widehat{\theta}_T)}\frac{\Delta_{t-k}}{g_{t-k}(\widehat{\theta}_T)}\\
&+\frac{1}{\sqrt{T}}\sum_{t=k+1}^{T}(u_t^2+\Delta_t)S_t(\widehat{\theta}_T)\frac{\Delta_{t-k}}{g_{t-k}(\widehat{\theta}_T)}+\frac{1}{\sqrt{T}}\sum_{t=k+1}^{T}(u_{t-k}^2+\Delta_{t-k})S_{t-k}\frac{\Delta_t}{g_t(\widehat{\theta}_T)}\\
:=&R_{241}+R_{242}+R_{243}+R_{244}.
\end{aligned}
$$

For simplicity, we only prove that $R_{241}=o_p(1)$. Decompose $R_{241}=\sum_{i=1}^4 R_{241i}$, where

$$
\begin{aligned}
R_{2411} =&\frac{1}{\sqrt{T}}\sum_{t=k+1}^{T}u_t^2S_t(\widehat{\theta}_T)u_{t-k}^2S_{t-k}(\widehat{\theta}_T), \quad R_{2412}=\frac{1}{\sqrt{T}}\sum_{t=k+1}^{T}\Delta_tS_t(\widehat{\theta}_T)\Delta_{t-k}S_{t-k}(\widehat{\theta}_T),\\
R_{2413} =&\frac{1}{\sqrt{T}}\sum_{t=k+1}^{T}u_t^2S_t(\widehat{\theta}_T)\Delta_{t-k}S_{t-k}(\widehat{\theta}_T), \quad R_{2414}=\frac{1}{\sqrt{T}}\sum_{t=k+1}^{T}\Delta_tS_t(\widehat{\theta}_T)u_{t-k}^2S_{t-k}(\widehat{\theta}_T).
\end{aligned}
$$

By noting that $S_t(\widehat{\theta}_T)=\frac{1}{g_t(\widehat{\theta}_T)}\frac{g_t(\widehat{\theta}_T)-\widehat{g}_t(\widehat{\theta}_T)}{\widehat{g}_t(\widehat{\theta}_T)}$, we can show

$$
\begin{aligned}
E|R_{2411}| \le&\frac{1}{\sqrt{T}}\sum_{t=k+1}^{T}E\Big|\frac{u_t^2}{g_t(\widehat{\theta}_T)}\frac{g_t(\widehat{\theta}_T)-\widehat{g}_t(\widehat{\theta}_T)}{\widehat{g}_t(\widehat{\theta}_T)}\frac{u_{t-k}^2}{g_{t-k}(\widehat{\theta}_T)}\frac{g_{t-k}(\widehat{\theta}_T)-\widehat{g}_{t-k}(\widehat{\theta}_T)}{\widehat{g}_{t-k}(\widehat{\theta}_T)}\Big|\\
\le&\frac{1}{\sqrt{T}}\sum_{t=k+1}^{T}\Big\|\frac{u_t^2}{g_t(\widehat{\theta}_T)}\Big\|_4\Big\|\frac{u_{t-k}^2}{g_{t-k}(\widehat{\theta}_T)}\Big\|_4 C^2(\kappa_T+\rho^t)^2=o(1),
\end{aligned}
$$

where the first inequality holds by triangular inequality, and the second inequality holds by Hölder's inequality and (B.15). Hence, it follows that $R_{2411}=o_p(1)$. Further, by (B.6) and the similar arguments as for $R_{2411}$, we can show that $R_{241i}=o_p(1)$ for $i=2,3,4$, which entails that $R_{241}=o_p(1)$ by Markov's inequality. □

Proof of Lemma A.14. Decompose $R_3=\sum_{i=1}^4 R_{3i}$, where

$$
\begin{aligned}
R_{31} =&\frac{1}{\sqrt{T}}\sum_{t=k+1}^{T}(\eta_t^2-1)\Big\{\frac{u_{t-k}^2}{g_{t-k}(\widehat{\theta}_T)}-\frac{u_{t-k}^2}{g_{t-k}(\theta_0)}\Big\},\\
R_{32} =&\frac{1}{\sqrt{T}}\sum_{t=k+1}^{T}(\eta_t^2-1)\frac{u_{t-k}^2}{g_{t-k}(\widehat{\theta}_T)}\frac{g_{t-k}(\widehat{\theta}_T)-\widehat{g}_{t-k}(\widehat{\theta}_T)}{\widehat{g}_{t-k}(\widehat{\theta}_T)},\\
R_{33} =&\frac{1}{\sqrt{T}}\sum_{t=k+1}^{T}(\eta_t^2-1)\frac{\Delta_{t-k}}{g_{t-k}(\widehat{\theta}_T)},\\
R_{34} =&\frac{1}{\sqrt{T}}\sum_{t=k+1}^{T}(\eta_t^2-1)\frac{\Delta_{t-k}}{g_{t-k}(\widehat{\theta}_T)}\frac{g_{t-k}(\widehat{\theta}_T)-\widehat{g}_{t-k}(\widehat{\theta}_T)}{\widehat{g}_{t-k}(\widehat{\theta}_T)}.
\end{aligned}
$$

The result follows by the following quantities:

(i) $R_{31} = o_p(1)$; (ii) $R_{32} = o_p(1)$; (iii) $R_{33} = o_p(1)$; (iv) $R_{34} = o_p(1)$.

(i) By Taylor's expansion and ergodic theorem, it is easy to show that $R_{31} = o_p(1)$.

(ii) By Taylor's expansion and the similar arguments as for part (i) in Lemma A.13, we have

$$\begin{aligned} R_{32} =& \frac{1}{\sqrt{T}} \sum_{t=k+1}^{T} (\eta_t^2 - 1) \frac{u_{t-k}}{g_{t-k}(\theta_0)} \frac{g_{t-k}(\widehat{\theta}_T) - \widehat{g}_{t-k}(\widehat{\theta}_T)}{\widehat{g}_{t-k}(\widehat{\theta}_T)} + o_p(1) \\ =& \frac{1}{\sqrt{T}} \sum_{t=k+1}^{T} (\eta_t^2 - 1)\eta_{t-k}^2 \frac{g_{t-k}(\widehat{\theta}_T) - \widehat{g}_{t-k}(\widehat{\theta}_T)}{g_{t-k}(\widehat{\theta}_T)} \\ &+ \frac{1}{\sqrt{T}} \sum_{t=k+1}^{T} (\eta_t^2 - 1)\eta_{t-k}^2 \frac{\{g_{t-k}(\widehat{\theta}_T) - \widehat{g}_{t-k}(\widehat{\theta}_T)\}^2}{g_{t-k}(\widehat{\theta}_T)\widehat{g}_{t-k}(\widehat{\theta}_T)} + o_p(1). \end{aligned} \tag{B.16}$$

By (B.15), we can show that the second term in (B.16) is $o_p(1)$, and hence,

$$R_{32} = \frac{1}{\sqrt{T}} \sum_{t=k+1}^{T} (\eta_t^2 - 1)\eta_{t-k}^2 \frac{g_{t-k}(\widehat{\theta}_T) - \widehat{g}_{t-k}(\widehat{\theta}_T)}{g_{t-k}(\widehat{\theta}_T)} + o_p(1).$$

Using Taylor's expansion, we have

$$R_{32} = R_{321} + \sqrt{T}(\widehat{\theta}_T - \theta_0) R_{322} + o_p(1)$$

for some $\theta^*$ lying between $\widehat{\theta}_T$ and $\theta_0$, where

$$\begin{aligned} R_{321} &= \frac{1}{\sqrt{T}} \sum_{t=k+1}^{T} (\eta_t^2 - 1)\eta_{t-k}^2 \frac{g_{t-k}(\theta_0) - \widehat{g}_{t-k}(\theta_0)}{g_{t-k}(\theta_0)}, \\ R_{322} &= \frac{1}{T} \sum_{t=k+1}^{T} (\eta_t^2 - 1)\eta_{t-k}^2 \frac{\{\frac{\partial g_{t-k}(\theta^*)}{\partial \theta} - \frac{\partial \widehat{g}_{t-k}(\theta^*)}{\partial \theta}\} g_{t-k}(\theta^*) - \frac{\partial g_{t-k}(\theta^*)}{\partial \theta}\{g_{t-k}(\theta^*) - \widehat{g}_{t-k}(\theta^*)\}}{g_{t-k}^2(\theta^*)}. \end{aligned}$$

By Lemmas A.3–A.4, it is not hard to show

$$R_{321} = \frac{1}{\sqrt{T}} \sum_{t=k+1}^{T} (\eta_t^2 - 1)\eta_{t-k}^2 \frac{\widetilde{g}_{t-k}(\theta_0) - \widehat{g}_{t-k}(\theta_0)}{g_{t-k}(\theta_0)} + o_p(1)$$

and $R_{322} = o_p(1)$. By the similar arguments as for Lemma A.10, we can get that $R_{321} = o_p(1)$ and thus $R_{32} = o_p(1)$.

(iii) By Taylor's expansion and the similar arguments as for part (i) in Lemma A.13, we have

$$R_{33} = \frac{1}{\sqrt{T}} \sum_{t=k+1}^{T} (\eta_t^2 - 1) \frac{\Delta_{t-k}}{g_{t-k}(\theta_0)} + o_p(1) = \frac{1}{\sqrt{T}} \sum_{t=k+1}^{T} (\eta_t^2 - 1)\eta_{t-k}^2 \frac{\tau_{t-k} - \widehat{\tau}_{t-k}}{\tau_{t-k}} + o_p(1).$$

Then, the result follows by the similar arguments as for part (ii).

(iv) The result follows directly by (B.15) and Lemma A.2(i). □

Proof of Lemma A.15. Decompose $R_4 = \sum_{i=1}^{4} R_{4i}$, where

$$R_{41} = \frac{1}{\sqrt{T}} \sum_{t=k+1}^{T} (\eta_{t-k}^2 - 1)\Big\{\frac{u_t^2}{g_t(\widehat{\theta}_T)} - \frac{u_t^2}{g_t(\theta_0)}\Big\},$$

$$R_{42} = \frac{1}{\sqrt{T}} \sum_{t=k+1}^{T} (\eta_{t-k}^2 - 1)\frac{u_t^2}{g_t(\widehat{\theta}_T)} \frac{g_t(\widehat{\theta}_T) - \widehat{g}_t(\widehat{\theta}_T)}{\widehat{g}_t(\widehat{\theta}_T)},$$

$$R_{43} = \frac{1}{\sqrt{T}} \sum_{t=k+1}^{T} (\eta_{t-k}^2 - 1)\frac{\Delta_t}{g_t(\widehat{\theta}_T)},$$

$$R_{44} = \frac{1}{\sqrt{T}} \sum_{t=k+1}^{T} (\eta_{t-k}^2 - 1)\frac{\Delta_t}{g_t(\widehat{\theta}_T)} \frac{g_t(\widehat{\theta}_T) - \widehat{g}_t(\widehat{\theta}_T)}{\widehat{g}_t(\widehat{\theta}_T)}.$$

The result follows by the following quantities:

(i) $R_{41} = -D_k\sqrt{T}(\widehat{\theta}_T - \theta_0) + o_p(1)$; (ii) $R_{42} = -\frac{\omega_0}{\gamma_0} H_k\big(\frac{1}{\sqrt{T}}\sum_{t=1}^{T} z_t\big) + o_p(1)$; (iii) $R_{43} = o_p(1)$; (iv) $R_{44} = o_p(1)$.

(i) By Taylor's expansion, we have

$$\begin{aligned} R_{41} &= -\Big\{\frac{1}{T}\sum_{t=k+1}^{T} (\eta_{t-k}^2 - 1)\frac{u_t^2}{g_t(\theta^*)}\frac{1}{g_t(\theta^*)}\frac{\partial g_t(\theta^*)}{\partial\theta}\Big\}\sqrt{T}(\widehat{\theta}_T - \theta_0) \\ &= -D_k\sqrt{T}(\widehat{\theta}_T - \theta_0) + o_p(1) \end{aligned}$$

for some $\theta^*$ lying between $\widehat{\theta}_T$ and $\theta_0$, where the last equality holds by the ergodic and continuous mapping theorems.

(ii) By the similar arguments as for (B.16), we have

$$R_{42} = \frac{1}{\sqrt{T}} \sum_{t=k+1}^{T} (\eta_{t-k}^2 - 1)\eta_t^2 \frac{\widetilde{g}_t(\theta_0) - \widehat{g}_t(\theta_0)}{g_t(\theta_0)} + o_p(1).$$

By (B.3), we can obtain

$$R_{42} = -\frac{1}{\sqrt{T}} \sum_{t=k+1}^{T} (\eta_{t-k}^2 - 1)\eta_t^2 g_t^{-1} \sum_{s=0}^{t-q-1} B_0^s(1,1)\sum_{i=1}^{q}\alpha_{i0}\Delta_{t-s-i}.$$

The result follows, since the similar arguments as for Lemma A.11 give us

$$\begin{aligned} R_{42} &= \sum_{s=0}^{\infty} B_0^s(1,1)\sum_{i=1}^{q}\alpha_{i0}E\Big\{g_t^{-1}u_{t-s-i}^2\eta_t^2(\eta_{t-k}^2 - 1)\Big\}\Big(\frac{1}{\sqrt{T}}\sum_{t=1}^{T} z_t\Big) + o_p(1) \\ &= E\Big\{g_t^{-1}\Big(g_t - \frac{\omega_0}{\gamma_0}\Big)\eta_t^2(\eta_{t-k}^2 - 1)\Big\}\Big(\frac{1}{\sqrt{T}}\sum_{t=1}^{T} z_t\Big) + o_p(1) \end{aligned}$$

$$= -\frac{\omega_0}{\gamma_0} H_k \Big( \frac{1}{\sqrt{T}} \sum_{t=1}^{T} z_t \Big) + o_p(1).$$

(iii) By the similar arguments as for Lemma A.11, we can show

$$R_{43} = \frac{1}{\sqrt{T}} \sum_{t=k+1}^{T} (\eta_{t-k}^2 - 1) \frac{\Delta_t}{g_t(\widehat{\theta}_T)} = E\{\eta_t^2(1-\eta_{t-k}^2)\} \Big( \frac{1}{\sqrt{T}} \sum_{t=1}^{T} z_t \Big) + o_p(1) = o_p(1).$$

(iv) It is straightforward to show that $R_{44} = o_p(1)$. □

Proof of Theorem 5.1. By Taylor's expansion and the similar arguments as for Theorem 2 in Hafner and Linton (2010), we can show

$$\begin{aligned} \breve{\tau}(x) - \tau(x) = & - \Big[ \frac{1}{T} \sum_{t=1}^{T} K_h(x - t/T) \frac{\partial^2 l_t(\tau, \theta_0)}{\partial \tau^2} \Big]^{-1} \Big[ \frac{1}{T} \sum_{t=1}^{T} K_h(x - t/T) \frac{\partial l_t(\tau, \theta_0)}{\partial \tau} \Big] \\ & + o_p(|\widehat{\tau}(x) - \tau(x)|), \end{aligned}$$

where $l_t(\tau, \theta_0) = \log(g_t) + \log(\tau) + \frac{y_t^2}{\tau g_t}$. Next, we can see

$$\frac{1}{T} \sum_{t=1}^{T} K_h(x - t/T) \frac{\partial^2 l_t(\tau, \theta_0)}{\partial \tau^2} = \tau(x)^{-2} \frac{1}{T} \sum_{t=1}^{T} K_h(x - t/T)(2\eta_t^2 - 1) = \tau(x)^{-2}(1 + o_p(1)),$$

and hence, it follows that

$$\breve{\tau}(x) - \tau(x) = \tau(x) \frac{1}{T} \sum_{t=1}^{T} K_h(x - t/T)(\eta_t^2 - 1) + o_p(\|\widehat{\tau}(x) - \tau(x)\|).$$

Third, by Taylor's expansion again we have[1]

$$\sqrt{T}(\breve{\theta}_T - \theta_0) = -\Big[ \frac{1}{T} \frac{\partial^2 \breve{L}_T^*(\theta_0)}{\partial \theta \partial \theta'} \Big]^{-1} \Big[ \frac{1}{\sqrt{T}} \frac{\partial \breve{L}_T^*(\theta_0)}{\partial \theta} \Big] + o_p(1),$$

where $\frac{1}{T} \frac{\partial^2 \breve{L}_T^*(\theta_0)}{\partial \theta \partial \theta'} \to_p E\Big[ \frac{\partial^2 L_T^*(\theta_0)}{\partial \theta \partial \theta'} \Big]$ by using the consistency of $\breve{\tau}(x)$. To deal with $\frac{1}{\sqrt{T}} \frac{\partial \breve{L}_T^*(\theta_0)}{\partial \theta}$, we use the similar arguments as in (A.4) and the similar arguments as for the proof of Theorem 2.2. Specifically, since $\breve{G}_T(\theta_0) \to_p E\psi_t$, we can obtain

$$\begin{aligned} \frac{1}{\sqrt{T}} \frac{\partial \breve{L}_T^*(\theta_0)}{\partial \theta} = & \frac{1}{\sqrt{T}} \sum_{t=1}^{T} (\psi_t - E\psi_t)(1 - \eta_t^2) - \frac{1}{\sqrt{T}} \sum_{t=1}^{T} (\psi_t - E\psi_t) u_t^2 (\breve{g}_t^{-1} - g_t^{-1}) \\ & - \frac{1}{\sqrt{T}} \sum_{t=1}^{T} (\breve{u}_t^2 - u_t^2) g_t^{-1} (\psi_t - E\psi_t) + o_p(1) \end{aligned}$$

[1]At this stage, we can not follow the proof of Theorem 3 in Hafner and Linton (2010) to remove the widecheck sign "ˇ" on the likelihood function, since we only expand the parametric part instead of the nonparametric part.

$$:= U_{13} + U_{14} + U_{15} + o_p(1).$$

Then, by Lemma B.1 below, it follows that

$$\frac{1}{\sqrt{T}}\frac{\partial \breve{L}_T^*(\theta_0)}{\partial\theta} = \frac{1}{\sqrt{T}}\sum_{t=1}^{T}\Big(\psi_t - E\psi_t + \frac{\omega_0}{\gamma_0}\Big[Eg_t^{-1}E\psi_t - Eg_t^{-1}\psi_t\Big]\Big)(1-\eta_t^2) + o_p(1).$$

Now, the conclusion follows by the martingale central limit theorem in Hall and Heyde (1980). □

LEMMA B.1. *Under the conditions of Theorem 5.1,* $U_{14} + U_{15} = \frac{\omega_0}{\gamma_0}\big[Eg_t^{-1}E\psi_t - Eg_t^{-1}\psi_t\big]\frac{1}{\sqrt{T}}\sum_{s=1}^{T}(1-\eta_s^2) + o_p(1)$.

PROOF OF LEMMA B.1. First, by using the similar arguments as in Lemma A.2, we have

$$\breve{u}_t^2 - u_t^2 = \tau_t^{-1}(\tau_t - \breve{\tau}_t)u_t^2 + O_p(\kappa_T^2)u_t^2. \tag{B.17}$$

Next, we can show

$$\begin{aligned}U_{14} &= \frac{1}{\sqrt{T}}\sum_{t=1}^{T}(\psi_t - E\psi_t)\eta_t^2\breve{g}_t^{-1}(\breve{g}_t - g_t) + o_p(1)\\ &= \frac{1}{\sqrt{T}}\sum_{t=1}^{T}(\psi_t - E\psi_t)(\eta_t^2-1)\breve{g}_t^{-1}\Big\{\sum_{k=0}^{\infty}B_0^k(1,1)\big(\sum_{i=1}^{q}\alpha_{i0}(\breve{u}_t^2 - u_t^2)\big)\Big\} + o_p(1)\\ &\quad + \frac{1}{\sqrt{T}}\sum_{t=1}^{T}(\psi_t - E\psi_t)\breve{g}_t^{-1}\Big\{\sum_{k=0}^{\infty}B_0^k(1,1)\big(\sum_{i=1}^{q}\alpha_{i0}(\breve{u}_t^2 - u_t^2)\big)\Big\} + o_p(1)\\ &=: U_{141} + U_{142} + o_p(1).\end{aligned}$$

By using similar arguments as for Lemma A.10, we can prove that $U_{141} = o_p(1)$. Moreover, by (B.17) and the similar arguments as for Lemma A.11, we have

$$\begin{aligned}U_{14} &= U_{142} + o_p(1)\\ &= \frac{1}{\sqrt{T}}\sum_{t=1}^{T}(\psi_t - E\psi_t)g_t^{-1}\Big(g_t - \frac{\omega_0}{\gamma_0}\Big)\tau_t^{-1}(\tau_t - \breve{\tau}_t) + o_p(1)\\ &= \frac{\omega_0}{\gamma_0}\Big[Eg_t^{-1}E\psi_t - Eg_t^{-1}\psi_t\Big]\frac{1}{\sqrt{T}}\sum_{t=1}^{T}\tau_t^{-1}(\tau_t - \breve{\tau}_t)\\ &\quad + \frac{1}{\sqrt{T}}\sum_{t=1}^{T}\Big\{(\psi_t - E\psi_t)\Big(1 - g_t^{-1}\frac{\omega_0}{\gamma_0}\Big) - \frac{\omega_0}{\gamma_0}\Big[Eg_t^{-1}E\psi_t - Eg_t^{-1}\psi_t\Big]\Big\}\tau_t^{-1}(\tau_t - \breve{\tau}_t) + o_p(1).\end{aligned}$$

Then, by using Proposition A.1 with $a_t = (\eta_t^2 - 1)$, $b_t = \big\{(\psi_t - E\psi_t)(1 - g_t^{-1}\frac{\omega_0}{\gamma_0}) - \frac{\omega_0}{\gamma_0}\big[Eg_t^{-1}E\psi_t - Eg_t^{-1}\psi_t\big]\big\}$ and $c_t = (u_t^2, g_t, \frac{\partial g_t}{\partial\theta'})$, we can prove that the second term in the last equation is $o_p(1)$, and hence,

$$
\begin{aligned}
U_{14} =& \frac{\omega_0}{\gamma_0}\Big[Eg_t^{-1}E\psi_t - Eg_t^{-1}\psi_t\Big]\frac{1}{\sqrt{T}}\sum_{t=1}^{T}\tau_t^{-1}(\tau_t - \breve{\tau}_t) + o_p(1) \\
=& \frac{\omega_0}{\gamma_0}\Big[Eg_t^{-1}E\psi_t - Eg_t^{-1}\psi_t\Big]\frac{1}{\sqrt{T}}\sum_{t=1}^{T}\Big(\frac{1}{Th}\sum_{s=1}^{T}K\Big(\frac{t-s}{Th}\Big)(1-\eta_s^2) + o_p(\|\widehat{\tau}_t - \tau_t\|)\Big) + o_p(1) \\
=& \frac{\omega_0}{\gamma_0}\Big[Eg_t^{-1}E\psi_t - Eg_t^{-1}\psi_t\Big]\frac{1}{\sqrt{T}}\sum_{s=1}^{T}(1-\eta_s^2)\frac{1}{Th}\sum_{t=1}^{T}K\Big(\frac{t-s}{Th}\Big) + o_p(1) \\
=& \frac{\omega_0}{\gamma_0}\Big[Eg_t^{-1}E\psi_t - Eg_t^{-1}\psi_t\Big]\frac{1}{\sqrt{T}}\sum_{s=1}^{T}(1-\eta_s^2) + o_p(1).
\end{aligned}
$$

Finally, the similar arguments imply

$$
U_{15} = \frac{1}{\sqrt{T}}\sum_{t=1}^{T}(\psi_t - E\psi_t)\tau_t^{-1}(\breve{\tau}_t - \tau_t) = o_p(1).
$$

This completes the proof. □

## APPENDIX C: ASSUMPTIONS AND PROOFS FOR THEOREM 6.1

To prove Theorem 6.1, we need the following assumptions.

ASSUMPTION C.1. *$W := I_N - \sum_{i=1}^{q} A_iA_i' - \sum_{j=1}^{p} B_jB_j'$ is positive definite.*

ASSUMPTION C.2. *(i) $\boldsymbol{\tau}(x)$ is bounded, positively definite and twice continuously differentiate on $x \in [0,1]$; (ii) $\underline{\tau} \le \inf_{x\in[0,1]}\|\boldsymbol{\tau}\| \le \sup_{x\in[0,1]}\|\boldsymbol{\tau}\| \le \overline{\tau}$, where $0 < \underline{\tau} \le \overline{\tau} < \infty$ are two constants.*

ASSUMPTION C.3. (i) *$K : [-1,1] \to \mathbb{R}_+$ is symmetric about zero, bounded and Lipschitz continuous with $\int_{-1}^{1} K(x)dx = 1$ and $C_r = \int_{-1}^{1} x^r K(x)dx$;* (ii) *$h \to 0$ and $Th \to \infty$ as $T \to \infty$.*

ASSUMPTION C.4. *$E\boldsymbol{\eta}_t\boldsymbol{\eta}_t' = I_N$, and $E\|\boldsymbol{\eta}_t\|^{12(1+\delta)} < \infty$.*

ASSUMPTION C.5. *(i) The process $\{\mathbf{u}_t\}$ is strictly stationary and ergodic; (ii) $\{\mathbf{u}_t\}$ is $\beta$-mixing with mixing coefficients $\beta(j)$ satisfying $\sum_{j=1}^{\infty} j^2\beta(j)^{\delta/(1+\delta)} < \infty$ for some $0 < \delta < 1$; (iii)$E\|\mathbf{u}_t\|^{12(1+\delta)} < \infty$.*

Assumption C.6. *The parameter space* $\boldsymbol{\Theta}$ *is compact, and the true parameter* $\boldsymbol{\theta}_0$ *is an interior point of* $\boldsymbol{\Theta}$.

Assumption C.7. *For* $\boldsymbol{\theta} \in \boldsymbol{\Theta}$*, if* $\boldsymbol{\theta} \neq \boldsymbol{\theta}_0$*, then* $\mathbf{g}_t(\boldsymbol{\theta}) \neq \mathbf{g}_t(\boldsymbol{\theta}_0)$ *almost surely for all* $t$.

Let $\mathcal{G}_t = \text{vec}(\mathbf{g}_t)$ and $\mathcal{U}_t = \text{vec}(\mathbf{u}_t\mathbf{u}_t')$. Recall $\mathcal{A}_i = A_i^{\otimes 2}$ and $\mathcal{B}_j = B_j^{\otimes 2}$. By (6.2), we have

$$\text{vec}(\mathbf{g}_t) = \text{vec}(W) + \sum_{i=1}^{q} \mathcal{A}_i \text{vec}(\mathbf{u}_{t-i}\mathbf{u}_{t-i}') + \sum_{j=1}^{p} \mathcal{B}_j \text{vec}(\mathbf{g}_{t-j}).$$

Then, by letting $\mathbb{G}_t = \Big(\mathcal{G}_t', \mathcal{G}_{t-1}', \cdots, \mathcal{G}_{t-p+1}'\Big)'$ and $\mathbb{C}_t = \Big(\big[\text{vec}(W) + \sum_{i=1}^{q} \mathcal{A}_i \mathcal{U}_{t-i}\big]', 0, \cdots, 0\Big)'$, it follows that

$$\mathbb{G}_t = \mathbb{C}_t + \mathbb{B}\mathbb{G}_{t-1}. \tag{C.1}$$

With a little abuse the notation, we denote $\Delta_{t-k-i} = \widehat{\mathcal{U}}_{t-k-i} - \mathcal{U}_{t-k-i}$, $\mathbf{b}(x) = C_2\boldsymbol{\tau}''(x)$, $\mathbf{v}_t(x) = \boldsymbol{\tau}(x)^{1/2}(\mathbf{u}_t\mathbf{u}_t' - I_N)\boldsymbol{\tau}(x)^{1/2}$, $\widetilde{\mathbf{S}}_t(\boldsymbol{\theta}) = \widehat{\mathbf{g}}_t^{-1}(\boldsymbol{\theta}) - \widetilde{\mathbf{g}}_t^{-1}(\boldsymbol{\theta})$, $\widehat{\mathcal{G}}_t = \text{vec}(\widehat{\mathbf{g}}_t)$ and $\widetilde{\mathcal{G}}_t = \text{vec}(\widetilde{\mathbf{g}}_t)$, where $\widetilde{\mathbf{g}}_t(\boldsymbol{\theta})$ is defined in the same way as $\widehat{\mathbf{g}}_t(\boldsymbol{\theta})$ with $\widehat{\mathbf{u}}_t$ replaced by $\mathbf{u}_t$. The following lemmas for the multivariate case are counterparts of Lemmas A.1–A.5.

Lemma C.1. *Suppose Assumptions C.1–C.7 hold. Then, almost surely (a.s.),*

(i) $\sup_{x\in(0,1)} \Big\|\widehat{\boldsymbol{\tau}}(x) - \boldsymbol{\tau}(x) - \frac{1}{T}\sum_{t=1}^{T} K_h\Big(x - \frac{t}{T}\Big)\mathbf{v}_t(x) - h^2\mathbf{b}(x)\Big\| = O\Big(\frac{\log T}{Th}\Big) + o(h^2)$;

(ii) $\sup_{x\in(0,1)} \Big|\frac{1}{T}\sum_{t=1}^{T} K_h\Big(x - \frac{t}{T}\Big)\mathbf{v}_t(x)\Big| = O\Big(\sqrt{\frac{\log T}{Th}}\Big)$.

Lemma C.2. *Suppose Assumptions C.1–C.7 hold. Then,*

(i) $\text{vec}^{-1}(\Delta_t) = \frac{1}{2}\boldsymbol{\tau}_t^{-3/4}(\boldsymbol{\tau}_t - \widehat{\boldsymbol{\tau}}_t)\boldsymbol{\tau}_t^{-1/4}\mathbf{u}_t\mathbf{u}_t' + \frac{1}{2}\mathbf{u}_t\mathbf{u}_t'\boldsymbol{\tau}_t^{-1/4}(\boldsymbol{\tau}_t - \widehat{\boldsymbol{\tau}}_t)\boldsymbol{\tau}_t^{-3/4} + O(\kappa_T^2)\mathbf{u}_t\mathbf{u}_t'$*, where* $O(1)$ *holds uniformly in* $t$*;*

(ii) $\sup_{\theta\in\Theta} \|\widetilde{\mathbf{S}}_t(\boldsymbol{\theta})\| \leq C\kappa_T$.

Lemma C.3. *Suppose Assumptions C.1–C.7 hold. Then, for any* $\iota \leq 6(1+\delta)$ *and all* $i, j = 1, 2, ..., \dim(\boldsymbol{\theta})$,

(i) $\sup_{\boldsymbol{\theta}\in\boldsymbol{\Theta}} \Big\|\widehat{\mathcal{G}}_t(\boldsymbol{\theta}) - \widetilde{\mathcal{G}}_t(\boldsymbol{\theta})\Big\|_\iota \leq C\kappa_T$;

(ii) $\sup_{\boldsymbol{\theta}\in\boldsymbol{\Theta}} \Big\|\frac{\partial\widehat{\mathcal{G}}_t(\boldsymbol{\theta})}{\partial\boldsymbol{\theta}_i} - \frac{\partial\widetilde{\mathcal{G}}_t(\boldsymbol{\theta})}{\partial\boldsymbol{\theta}_i}\Big\|_\iota \leq C\kappa_T$;

(iii) $\sup_{\boldsymbol{\theta}\in\boldsymbol{\Theta}} \Big\|\frac{\partial^2\widehat{\mathcal{G}}_t(\boldsymbol{\theta})}{\partial\boldsymbol{\theta}_i\partial\boldsymbol{\theta}_j} - \frac{\partial^2\widetilde{\mathcal{G}}_t(\boldsymbol{\theta})}{\partial\boldsymbol{\theta}_i\partial\boldsymbol{\theta}_j}\Big\|_\iota \leq C\kappa_T$.

Lemma C.4. *Suppose Assumptions C.1-C.7 hold. Then, there exists a $\rho \in (0,1)$ such that for any $\iota \leq 6(1+\delta)$ and all $i,j = 1,2,...,\dim(\boldsymbol{\theta})$,*

(i) $\sup_{\boldsymbol{\theta}\in\boldsymbol{\Theta}} \left\| \mathcal{G}_t(\boldsymbol{\theta}) - \widetilde{\mathcal{G}}_t(\boldsymbol{\theta}) \right\|_\iota \leq C\rho^t$;

(ii) $\sup_{\boldsymbol{\theta}\in\boldsymbol{\Theta}} \left\| \frac{\partial \mathcal{G}_t(\boldsymbol{\theta})}{\partial \boldsymbol{\theta}_i} - \frac{\partial \widetilde{\mathcal{G}}_t(\boldsymbol{\theta})}{\partial \boldsymbol{\theta}_i} \right\|_\iota \leq C\rho^t$;

(iii) $\sup_{\boldsymbol{\theta}\in\boldsymbol{\Theta}} \left\| \frac{\partial^2 \mathcal{G}_t(\boldsymbol{\theta})}{\partial \boldsymbol{\theta}_i \partial \boldsymbol{\theta}_j} - \frac{\partial^2 \widetilde{\mathcal{G}}_t(\boldsymbol{\theta})}{\partial \boldsymbol{\theta}_i \partial \boldsymbol{\theta}_j} \right\|_\iota \leq C\rho^t$.

Lemma C.5. *Suppose Assumptions C.1–C.7 hold. Then, $\{(\mathcal{U}_t, \mathcal{G}_t, \frac{\partial \mathcal{G}_t(\boldsymbol{\theta})}{\partial \boldsymbol{\theta}'})\}$ is strictly stationary and $\beta$-mixing with exponential decay.*

The ideas to prove the above lemmas are similar to the arguments used in the univariate case, and hence we only give the sketch of the proof in the sequel.

Proof of Lemma C.1. See the proof of Lemma 1 in Hafner and Linton (2010). □

Proof of Lemma C.2. (i) Observe that

$$\widehat{\boldsymbol{\tau}}(x) = \boldsymbol{\tau}(x)^{1/2}[I_N + \boldsymbol{\tau}(x)^{-1/2}(\widehat{\boldsymbol{\tau}}(x) - \boldsymbol{\tau}(x))\boldsymbol{\tau}(x)^{-1/2}]\boldsymbol{\tau}(x)^{1/2}.$$

By Taylor's expansion and Lemma C.1, we can show

$$\widehat{\boldsymbol{\tau}}(x)^{-1/2} = \boldsymbol{\tau}(x)^{-1/2} - \frac{1}{2}\boldsymbol{\tau}(x)^{-3/4}(\widehat{\boldsymbol{\tau}}(x) - \boldsymbol{\tau}(x))\boldsymbol{\tau}(x)^{-3/4} + O(\kappa_T^2).$$

Since $\mathrm{vec}^{-1}(\Delta_t) = \widehat{\mathbf{u}}_t\widehat{\mathbf{u}}_t' - \mathbf{u}_t\mathbf{u}_t = \widehat{\boldsymbol{\tau}}(x)^{-1/2}\mathbf{y}_t\mathbf{y}_t'\widehat{\boldsymbol{\tau}}(x)^{-1/2} - \boldsymbol{\tau}(x)^{-1/2}\mathbf{y}_t\mathbf{y}_t'\boldsymbol{\tau}(x)^{-1/2}$, the result follows.

(ii) It is clear that $\widetilde{\mathbf{S}}_t(\boldsymbol{\theta}) = \widehat{\mathbf{g}}_t^{-1}(\boldsymbol{\theta})[\widetilde{\mathbf{g}}_t(\boldsymbol{\theta}) - \widehat{\mathbf{g}}_t(\boldsymbol{\theta})]\widetilde{\mathbf{g}}_t^{-1}(\boldsymbol{\theta})$. By Assumptions C.1 and C.6, we have that $\sup_{\boldsymbol{\theta}\in\boldsymbol{\Theta}} \|\widetilde{\mathbf{g}}_t^{-1}(\boldsymbol{\theta})\| \leq \sup_{\boldsymbol{\theta}\in\boldsymbol{\Theta}} \|W^{-1}\| < \infty$, and similarly $\sup_{\boldsymbol{\theta}\in\boldsymbol{\Theta}} \|\widehat{\mathbf{g}}_t^{-1}(\boldsymbol{\theta})\| < \infty$. Hence, the result follows by Lemma C.3(i). □

Proof of Lemma C.3. We only prove the result (i), since the proofs for results (ii)–(iii) are similar.

Given constant initial values, by (C.1) and the similar arguments as for (B.3), we have

$$\widehat{\mathcal{G}}_t(\boldsymbol{\theta}) - \widetilde{\mathcal{G}}_t(\boldsymbol{\theta}) = \sum_{k=0}^{t-q-1} \mathbb{B}^k(1:N^2, 1:N^2)(\sum_{i=1}^{q} \mathcal{A}_i \Delta_{t-k-i}), \tag{C.2}$$

where $\mathbb{B}^k(1:N^2, 1:N^2)$ denotes the upper-left $N^2 \times N^2$ submatrix of $\mathbb{B}^k$. By Lemma C.2(i), we can show that $\|\Delta_t\|_\iota \leq C\kappa_T\|\mathcal{U}_t\|_\iota$. The result follows by noting $\sup_{\boldsymbol{\theta}\in\boldsymbol{\Theta}} \rho(\mathbb{B}) < 1$ and Minkowski's inequality. □

Proof of Lemma C.4. The results hold by using the similar arguments as for Theorem 3.2 in Francq and Zakoïan (2010), and hence the details are omitted. □

Proof of Lemma C.5. It follows the similar arguments as for Lemma A.5. □

To prove the asymptotic normality of $\widehat{\boldsymbol{\theta}}_T$, we can first show that

$$\widehat{\boldsymbol{\theta}}_T \to_p \boldsymbol{\theta}_0 \text{ as } T \to \infty,$$

by using the similar arguments as for Theorem 2.2(i). Next, we need an additional lemma below:

Lemma C.6. *Let $m_T$ be defined as in (A.10). Then, under the conditions in Theorem 6.1,*

$$\max_{1\le i\le m_T}\max_{i+1\le t\le T}\left\|\boldsymbol{\tau}_t^{-3/4}(\widehat{\boldsymbol{\tau}}_t-\boldsymbol{\tau}_t)\boldsymbol{\tau}_t^{-1/4}-\boldsymbol{\tau}_{t-i}^{-3/4}(\widehat{\boldsymbol{\tau}}_{t-i}-\boldsymbol{\tau}_{t-i})\boldsymbol{\tau}_{t-i}^{-1/4}\right\| = o\Big(\frac{1}{\sqrt{T}}\Big) \ a.s.$$

Proof of Lemma C.6. The proof is similar to the one for Lemma A.9. Specifically, we first notice

$$\begin{aligned}&\left\|\boldsymbol{\tau}_t^{-3/4}(\widehat{\boldsymbol{\tau}}_t-\boldsymbol{\tau}_t)\boldsymbol{\tau}_t^{-1/4}-\boldsymbol{\tau}_{t-i}^{-3/4}(\widehat{\boldsymbol{\tau}}_{t-i}-\boldsymbol{\tau}_{t-i})\boldsymbol{\tau}_{t-i}^{-1/4}\right\|\\ \le&\left\|\boldsymbol{\tau}_{t-i}^{-3/4}(\widehat{\boldsymbol{\tau}}_t-\widehat{\boldsymbol{\tau}}_{t-i})\boldsymbol{\tau}_{t-i}^{-1/4}\right\|+\left\|\boldsymbol{\tau}_t^{-3/4}\widehat{\boldsymbol{\tau}}_t\boldsymbol{\tau}_t^{-1/4}-\boldsymbol{\tau}_{t-i}^{-3/4}\widehat{\boldsymbol{\tau}}_t\boldsymbol{\tau}_{t-i}^{-1/4}\right\| := I_1+I_2.\end{aligned}$$

Then, we can show that for any $0 < s - s' < m_T$, we have $\|\widehat{\boldsymbol{\tau}}_s - \widehat{\boldsymbol{\tau}}_{s'}\| \le o(T^{-1/2})$ a.s. so that $I_1 = o(T^{-1/2})$. Furthermore, by Taylor's expansion we can obtain

$$\begin{aligned}\boldsymbol{\tau}_{t-i}^{-1/4} =&\boldsymbol{\tau}_t^{-1/8}[I_N+\boldsymbol{\tau}_t^{-1/2}(\boldsymbol{\tau}_{t-j}-\boldsymbol{\tau}_t)\boldsymbol{\tau}_t^{-1/2}]^{-1/4}\boldsymbol{\tau}_t^{-1/8}\\ =&\boldsymbol{\tau}_t^{-1/8}[I_N-\frac{1}{4}\boldsymbol{\tau}_t^{-1/2}(\boldsymbol{\tau}_{t-j}-\boldsymbol{\tau}_t)\boldsymbol{\tau}_t^{-1/2}]\boldsymbol{\tau}_t^{-1/8}+o(T^{-1})\\ =&\boldsymbol{\tau}_t^{-1/4}-\frac{1}{4}\boldsymbol{\tau}_t^{-5/8}(\boldsymbol{\tau}_{t-j}-\boldsymbol{\tau}_t)\boldsymbol{\tau}_t^{-5/8}+o(T^{-1})=\boldsymbol{\tau}_t^{-1/4}+o(T^{-1/2}),\end{aligned}$$

which entails that $I_2 = o(T^{-1/2})$. □

Third, similar to (A.4), we consider the following decomposition:

$$\frac{1}{\sqrt{T}}\frac{\partial\widehat{\mathbf{L}}_T(\boldsymbol{\theta}_0)}{\partial\boldsymbol{\theta}_m}=\sum_{i=1}^{12}\mathbf{U}_i, \tag{C.3}$$

where

$$\mathbf{U}_1=\frac{1}{\sqrt{T}}\sum_{t=1}^{T}\mathrm{tr}\Big[(I_N-\mathbf{u}_t\mathbf{u}_t'\widetilde{\mathbf{g}}_t^{-1})\frac{\partial\widetilde{\mathbf{g}}_t}{\partial\boldsymbol{\theta}_m}\widetilde{\mathbf{g}}_t^{-1}\Big],\ \mathbf{U}_2=\frac{1}{\sqrt{T}}\sum_{t=1}^{T}\mathrm{tr}\Big[(I_N-\mathbf{u}_t\mathbf{u}_t'\widetilde{\mathbf{g}}_t^{-1})(\frac{\partial\widehat{\mathbf{g}}_t}{\partial\boldsymbol{\theta}_m}-\frac{\partial\widetilde{\mathbf{g}}_t}{\partial\boldsymbol{\theta}_m})\widetilde{\mathbf{g}}_t^{-1}\Big],$$

$$\mathbf{U}_3 = \frac{1}{\sqrt{T}}\sum_{t=1}^{T}\mathrm{tr}\Big[(I_N - \mathbf{u}_t\mathbf{u}_t'\widetilde{\mathbf{g}}_t^{-1})\frac{\partial\widetilde{\mathbf{g}}_t}{\partial\boldsymbol{\theta}_m}\widetilde{\mathbf{S}}_t\Big], \quad \mathbf{U}_4 = \frac{1}{\sqrt{T}}\sum_{t=1}^{T}\mathrm{tr}\Big[(I_N - \mathbf{u}_t\mathbf{u}_t'\widetilde{\mathbf{g}}_t^{-1})(\frac{\partial\widehat{\mathbf{g}}_t}{\partial\boldsymbol{\theta}_m} - \frac{\partial\widetilde{\mathbf{g}}_t}{\partial\boldsymbol{\theta}_m})\widetilde{\mathbf{S}}_t\Big],$$

$$\mathbf{U}_5 = -\frac{1}{\sqrt{T}}\sum_{t=1}^{T}\mathrm{tr}\Big[\mathbf{u}_t\mathbf{u}_t'\widetilde{\mathbf{S}}_t\frac{\partial\widetilde{\mathbf{g}}_t}{\partial\boldsymbol{\theta}_m}\widetilde{\mathbf{g}}_t^{-1}\Big], \quad \mathbf{U}_6 = -\frac{1}{\sqrt{T}}\sum_{t=1}^{T}\mathrm{tr}\Big[\mathbf{u}_t\mathbf{u}_t'\widetilde{\mathbf{S}}_t(\frac{\partial\widehat{\mathbf{g}}_t}{\partial\boldsymbol{\theta}_m} - \frac{\partial\widetilde{\mathbf{g}}_t}{\partial\boldsymbol{\theta}_m})\widetilde{\mathbf{g}}_t^{-1}\Big],$$

$$\mathbf{U}_7 = -\frac{1}{\sqrt{T}}\sum_{t=1}^{T}\mathrm{tr}\Big[\mathbf{u}_t\mathbf{u}_t'\widetilde{\mathbf{S}}_t\frac{\partial\widetilde{\mathbf{g}}_t}{\partial\boldsymbol{\theta}_m}\widetilde{\mathbf{S}}_t\Big], \quad \mathbf{U}_8 = -\frac{1}{\sqrt{T}}\sum_{t=1}^{T}\mathrm{tr}\Big[\mathbf{u}_t\mathbf{u}_t'\widetilde{\mathbf{S}}_t(\frac{\partial\widehat{\mathbf{g}}_t}{\partial\boldsymbol{\theta}_m} - \frac{\partial\widetilde{\mathbf{g}}_t}{\partial\boldsymbol{\theta}_m})\widetilde{\mathbf{S}}_t\Big],$$

$$\mathbf{U}_9 = -\frac{1}{\sqrt{T}}\sum_{t=1}^{T}\mathrm{tr}\Big[\mathrm{vec}^{-1}(\Delta_t)\widetilde{\mathbf{g}}_t^{-1}\frac{\partial\widetilde{\mathbf{g}}_t}{\partial\boldsymbol{\theta}_m}\widetilde{\mathbf{g}}_t^{-1}\Big], \quad \mathbf{U}_{10} = -\frac{1}{\sqrt{T}}\sum_{t=1}^{T}\mathrm{tr}\Big[\mathrm{vec}^{-1}(\Delta_t)\widetilde{\mathbf{g}}_t^{-1}(\frac{\partial\widehat{\mathbf{g}}_t}{\partial\boldsymbol{\theta}_m} - \frac{\partial\widetilde{\mathbf{g}}_t}{\partial\boldsymbol{\theta}_m})\widetilde{\mathbf{g}}_t^{-1}\Big],$$

$$\mathbf{U}_{11} = -\frac{1}{\sqrt{T}}\sum_{t=1}^{T}\mathrm{tr}\Big[\mathrm{vec}^{-1}(\Delta_t)\widetilde{\mathbf{g}}_t^{-1}\frac{\partial\widetilde{\mathbf{g}}_t}{\partial\boldsymbol{\theta}_m}\widetilde{\mathbf{S}}_t\Big], \quad \mathbf{U}_{12} = -\frac{1}{\sqrt{T}}\sum_{t=1}^{T}\mathrm{tr}\Big[\mathrm{vec}^{-1}(\Delta_t)\widetilde{\mathbf{g}}_t^{-1}(\frac{\partial\widehat{\mathbf{g}}_t}{\partial\boldsymbol{\theta}_m} - \frac{\partial\widetilde{\mathbf{g}}_t}{\partial\boldsymbol{\theta}_m})\widetilde{\mathbf{S}}_t\Big].$$

Below, we need several lemmas to deal with $\mathbf{U}_i$.

LEMMA C.7. *Under the conditions in Theorem 6.1,* $\mathbf{U}_2 = o_p(1)$ *and* $\mathbf{U}_3 = o_p(1)$.

PROOF OF LEMMA C.7. By Lemma C.4, we can show

$$\begin{aligned}\mathbf{U}_3 =& -\frac{1}{\sqrt{T}}\sum_{t=1}^{T}\mathrm{tr}\Big[\mathbf{g}_t^{-1/2}(I_N - \boldsymbol{\eta}_t\boldsymbol{\eta}_t')\mathbf{g}_t^{-1/2}\frac{\partial\mathbf{g}_t}{\partial\theta_m}\mathbf{g}_t^{-1}(\widehat{\mathbf{g}}_t - \widetilde{\mathbf{g}}_t)\Big] + o_p(1)\\ =& -\frac{1}{\sqrt{T}}\sum_{t=1}^{T}\mathrm{vec}(\frac{\partial\mathbf{g}_t}{\partial\boldsymbol{\theta}_m})'[\mathbf{g}_t^{-1/2}(I_N - \boldsymbol{\eta}_t\boldsymbol{\eta}_t')\mathbf{g}_t^{-1/2}\otimes\mathbf{g}_t^{-1}]\mathrm{vec}(\widehat{\mathbf{g}}_t - \widetilde{\mathbf{g}}_t) + o_p(1).\end{aligned}$$

Then, by (C.2) we can obtain

$$\mathrm{vec}(\widehat{\mathbf{g}}_t - \widetilde{\mathbf{g}}_t) = \widehat{\mathcal{G}}_t - \widetilde{\mathcal{G}}_t = \sum_{k=0}^{t-q-1}\mathbb{B}_0^k(1:N^2, 1:N^2)(\sum_{i=1}^{q}\mathcal{A}_{i0}\Delta_{t-k-i}).$$

Hence,

$$\begin{aligned}\mathbf{U}_3 =& -\sum_{i=1}^{q}\frac{1}{\sqrt{T}}\sum_{t=1}^{T}\mathrm{vec}(\frac{\partial\mathbf{g}_t}{\partial\boldsymbol{\theta}_m})'[\mathbf{g}_t^{-1/2}(I_N - \boldsymbol{\eta}_t\boldsymbol{\eta}_t')\mathbf{g}_t^{-1/2}\otimes\mathbf{g}_t^{-1}]\\ &\times\Big[\sum_{k=0}^{t-q-1}\mathbb{B}_0^k(1:N^2, 1:N^2)\mathcal{A}_{i0}\Delta_{t-k-i}\Big] + o_p(1) =: \sum_{i=1}^{q}\mathbf{U}_{3i} + o_p(1).\end{aligned}$$

By letting $\boldsymbol{\varphi}_t' = \mathrm{vec}(\frac{\partial\mathbf{g}_t}{\partial\boldsymbol{\theta}_m})'[\mathbf{g}_t^{-1/2}(I_N - \boldsymbol{\eta}_t\boldsymbol{\eta}_t')\mathbf{g}_t^{-1/2}\otimes\mathbf{g}_t^{-1}]$, we have

$$\begin{aligned}\mathbf{U}_{3i} =& -\frac{1}{\sqrt{T}}\sum_{t=1}^{T}\boldsymbol{\varphi}_t'\Big[\sum_{k=0}^{t-q-1}\mathbb{B}_0^k(1:N^2, 1:N^2)\mathcal{A}_{i0}\Delta_{t-k-i}\Big]\\ =& -\frac{1}{\sqrt{T}}\sum_{k=0}^{T-q-1}\sum_{t=k+q+1}^{T}\boldsymbol{\varphi}_t'\Big[\mathbb{B}_0^k(1:N^2, 1:N^2)\mathcal{A}_{i0}\Delta_{t-k-i}\Big]\end{aligned}$$

$$
\begin{aligned}
&= -\frac{1}{\sqrt{T}}\sum_{k=0}^{m_T}\sum_{t=k+q+1}^{T}\boldsymbol{\varphi}_t'\Big[\mathbb{B}_0^k(1:N^2,1:N^2)\mathcal{A}_{i0}\Delta_{t-k-i}\Big]\\
&\quad -\frac{1}{\sqrt{T}}\sum_{k=m_T+1}^{T-q-1}\sum_{t=k+q+1}^{T}\boldsymbol{\varphi}_t'\Big[\mathbb{B}_0^k(1:N^2,1:N^2)\mathcal{A}_{i0}\Delta_{t-k-i}\Big] =: \mathbf{U}_{3i1}+\mathbf{U}_{3i2}.
\end{aligned}
$$

Note that $E\|\boldsymbol{\varphi}_t\|\sup_s\|\Delta_s\|<\infty$ by Hölder's inequality. Then, by using the fact $\rho(\mathbb{B}_0)<1$, we can show that $E\|\mathbf{U}_{3i2}\|\le O(\rho(\mathbb{B}_0)^{m_T})O(\sqrt{\frac{\log T}{h}})=o(1)$, which implies that $\mathbf{U}_{3i2}=o_p(1)$. So, it follows that

$$
\mathbf{U}_{3i} = -\frac{1}{\sqrt{T}}\sum_{k=0}^{m_T}\sum_{t=k+q+1}^{T}\boldsymbol{\varphi}_t'\Big[\mathbb{B}_0^k(1:N^2,1:N^2)\mathcal{A}_{i0}\Delta_{t-k-i}\Big]+o_p(1) =: \sum_{k=0}^{m_T}\mathbf{U}_{3ik}+o_p(1).
$$

Note that by using Lemma C.2(i), we can obtain

$$
\begin{aligned}
\Delta_t &= \frac{1}{2}\mathrm{vec}\Big(\boldsymbol{\tau}_t^{-3/4}(\boldsymbol{\tau}_t-\widehat{\boldsymbol{\tau}}_t)\boldsymbol{\tau}_t^{-1/4}\mathbf{u}_t\mathbf{u}_t'+\mathbf{u}_t\mathbf{u}_t'\boldsymbol{\tau}_t^{-1/4}(\boldsymbol{\tau}_t-\widehat{\boldsymbol{\tau}}_t)\boldsymbol{\tau}_t^{-3/4}\Big)+O_p(\kappa_T^2)\\
&= \frac{1}{2}\Big([\boldsymbol{\tau}_t^{-3/4}\otimes\mathbf{u}_t\mathbf{u}_t'\boldsymbol{\tau}_t^{-1/4}]+[\mathbf{u}_t\mathbf{u}_t'\boldsymbol{\tau}_t^{-1/4}\otimes\boldsymbol{\tau}_t^{-3/4}]\Big)\mathrm{vec}(\boldsymbol{\tau}_t-\widehat{\boldsymbol{\tau}}_t)+O_p(\kappa_T^2),
\end{aligned}
\tag{C.4}
$$

which entails

$$
\begin{aligned}
\mathbf{U}_{3i} &= -\frac{1}{\sqrt{T}}\sum_{k=0}^{m_T}\sum_{t=k+q+1}^{T}\boldsymbol{\varphi}_t'\Big[\mathbb{B}_0^k(1:N^2,1:N^2)\mathcal{A}_{i0}[\boldsymbol{\tau}_t^{-3/4}\otimes\mathbf{u}_{t-k-i}\mathbf{u}_{t-k-i}'\boldsymbol{\tau}_t^{-1/4}]\mathrm{vec}(\boldsymbol{\tau}_t-\widehat{\boldsymbol{\tau}}_t)\Big]\\
&\quad +o_p(1)\\
&= \sum_{k=0}^{m_T}\frac{1}{\sqrt{T}}\sum_{t=k+q+1}^{T}\boldsymbol{\varphi}_t'\mathbb{B}_0^k(1:N^2,1:N^2)\mathcal{A}_{i0}[I_N\otimes\mathbf{u}_{t-k-i}\mathbf{u}_{t-k-i}'][\boldsymbol{\tau}_t^{-3/4}\otimes\boldsymbol{\tau}_t^{-1/4}]\\
&\quad\times\mathrm{vec}\Big(\frac{1}{Th}\sum_{s=1}^{T}K\Big(\frac{t-s}{Th}\Big)\boldsymbol{\tau}_t^{1/2}(\mathbf{u}_s\mathbf{u}_s'-I_N)\boldsymbol{\tau}_t^{1/2}\Big)+o_p(1)\\
&= \sum_{k=0}^{m_T}\frac{1}{\sqrt{T}}\sum_{t=k+q+1}^{T}\boldsymbol{\varphi}_t'\mathbb{B}_0^k(1:N^2,1:N^2)\mathcal{A}_{i0}[I_N\otimes\mathbf{u}_{t-k-i}\mathbf{u}_{t-k-i}'][\boldsymbol{\tau}_t^{-1/4}\otimes\boldsymbol{\tau}_t^{1/4}]\\
&\quad\times\frac{1}{Th}\sum_{s=1}^{T}K\Big(\frac{t-s}{Th}\Big)\mathrm{vec}(\mathbf{u}_s\mathbf{u}_s'-I_N)+o_p(1) =: \sum_{k=0}^{m_T}\mathbf{U}_{3i,k}+o_p(1).
\end{aligned}
$$

For $\mathbf{U}_{3i,k}$, we first show

$$
E\|\boldsymbol{\varphi}_t'[I_N\otimes\mathbf{u}_{t-k-i}\mathbf{u}_{t-k-i}']\|^{3(1+2\delta)}<\infty
$$

as $E\|\mathrm{vec}(\mathbf{u}_t\mathbf{u}_t'-I_N)\|^{6(1+\delta)}<\infty$. By Hölder's inequality and the fact that $\sup_{\boldsymbol{\theta}\in\boldsymbol{\Theta}}\|\mathbf{g}_t^{-1}\|<$

$\infty$ and $I_N - \boldsymbol{\eta}_t\boldsymbol{\eta}_t'$ is independent of $\mathcal{F}_{t-1}$, we have

$$\begin{aligned}
&E\|\boldsymbol{\varphi}_t'[I_N \otimes \mathbf{u}_{t-k-i}\mathbf{u}_{t-k-i}']\|^{3(1+2\delta)}\\
\leq &CE\|\boldsymbol{\varphi}_t\|^{6(1+2\delta)}E\|I_N \otimes \mathbf{u}_{t-k-i}\mathbf{u}_{t-k-i}'\|^{6(1+2\delta)}\\
\leq &CE\|\mathrm{vec}(\mathbf{g}_t^{-1}\frac{\partial \mathbf{g}_t}{\partial \boldsymbol{\theta}}\mathbf{g}_t^{-1/2}(I_N - \boldsymbol{\eta}_t\boldsymbol{\eta}_t')\mathbf{g}_t^{-1/2})\|^{6(1+2\delta)}E\|I_N \otimes \mathbf{u}_{t-k-i}\mathbf{u}_{t-k-i}'\|^{6(1+2\delta)}\\
\leq &CE\|\frac{\partial \mathbf{g}_t}{\partial \theta}\|^{6(1+2\delta)}E\|I_N - \boldsymbol{\eta}_t\boldsymbol{\eta}_t'\|^{6(1+2\delta)}E\|I_N \otimes \mathbf{u}_{t-k-i}\mathbf{u}_{t-k-i}'\|^{6(1+2\delta)} < \infty.
\end{aligned} \tag{C.5}$$

Then, by using Proposition A.1 with $a_t = \mathrm{vec}(\mathbf{u}_t\mathbf{u}_t' - I_N)$, $b_t = \boldsymbol{\varphi}_t'\mathbb{B}_0^k(1:N^2, 1:N^2)\mathcal{A}_{i0}[I_N \otimes \mathbf{u}_{t-k-i}\mathbf{u}_{t-k-i}']$, and $c_t = \{\mathrm{vec}(I_N - \mathbf{u}_t\mathbf{u}_t'), \mathcal{G}_t, \frac{\partial \mathcal{G}_t}{\partial \boldsymbol{\theta}}\}$, it follows that for some $\rho \in (0,1)$, $\mathbf{U}_{3i,k} = o_p(\rho^k)$ uniformly in $k$. Hence, $\mathbf{U}_{3i} = o_p(1)$, implying that $\mathbf{U}_3 = o_p(1)$. Similarly, we can show that $\mathbf{U}_2 = o_p(1)$. □

We should mention that we need higher moments than the univariate GARCH case for $\mathbf{u}_t$, since it seems quite difficult to obtain the following recursive representation

$$\sum_{k=0}^{\infty}\mathbb{B}_0^k(1:N^2, 1:N^2)\sum_{i=1}^{q}\mathcal{A}_{i0}[I_N \otimes \mathbf{u}_{t-k-i}\mathbf{u}_{t-k-i}']$$

as a function of $\mathbf{g}_t$. In the univariate case, the above is reduced to $g_t - \gamma_0^{-1}\omega_0$ by (B.10), and so we don't need bound the term $I_N \otimes \mathbf{u}_{t-k-i}\mathbf{u}_{t-k-i}'$ in (C.5).

Lemma C.8. *Under the conditions in Theorem 6.1,* $\mathbf{U}_5 = -\frac{1}{\sqrt{T}}\sum_{t=1}^{T}\mathbf{M}_m[\boldsymbol{\tau}_t^{-1/4} \otimes \boldsymbol{\tau}_t^{1/4}]\mathrm{vec}(\mathbf{u}_t\mathbf{u}_t' - I_N) + o_p(1)$.

Proof of Lemma C.8. By the similar arguments as for Lemma C.7 and Proposition A.1, we can obtain

$$\begin{aligned}
\mathbf{U}_5 =&\frac{1}{\sqrt{T}}\sum_{t=1}^{T}\mathrm{tr}\Big[(\widehat{\mathbf{g}}_t - \widetilde{\mathbf{g}}_t){\mathbf{g}_t}^{-1}\frac{\partial \mathbf{g}_t}{\partial \boldsymbol{\theta}_m}{\mathbf{g}_t}^{-1}\Big] + o_p(1)\\
=&\frac{1}{\sqrt{T}}\sum_{t=1}^{T}\mathrm{vec}(\frac{\partial \mathbf{g}_t}{\partial \boldsymbol{\theta}_m})'[\mathbf{g}_t^{-1} \otimes {\mathbf{g}_t}^{-1}]\mathrm{vec}(\widehat{\mathbf{g}}_t - \widetilde{\mathbf{g}}_t) + o_p(1).
\end{aligned}$$

Next, by (C.2) and interchanging the summation, we have

$$\mathbf{U}_5 =\frac{1}{\sqrt{T}}\sum_{k=0}^{T-q-1}\Big[\mathbb{B}_0^k(1:N^2, 1:N^2)\Big(\sum_{i=1}^{q}\mathcal{A}_{i0}\Big)\Delta_{t-k-i}\Big]'(\mathbf{g}_t^{-1})^{\otimes 2}\sum_{t=k+q+1}^{T}\mathrm{vec}\Big(\frac{\partial \mathbf{g}_t}{\partial \boldsymbol{\theta}_m}\Big) + o_p(1).$$

Hence, by using $\kappa_T^2 = o(T^{-1/2})$ and some matrix algebra, we can obtain

$$\mathbf{U}_5 =\frac{1}{\sqrt{T}}\sum_{k=0}^{T-q-1}\Big[\mathbb{B}_0^k(1:N^2, 1:N^2)\Big(\sum_{i=1}^{q}\mathcal{A}_{i0}\Big)[\boldsymbol{\tau}_{t-k-i}^{-3/4} \otimes \mathbf{u}_{t-k-i}\mathbf{u}_{t-k-i}'\boldsymbol{\tau}_{t-k-i}^{-1/4}]\mathrm{vec}(\boldsymbol{\tau}_{t-k-i} - \widehat{\boldsymbol{\tau}}_{t-k-i})\Big]'$$

$$\times \sum_{t=k+q+1}^{T} (\mathbf{g}_t^{-1})^{\otimes 2} \text{vec}\Big(\frac{\partial \mathbf{g}_t}{\partial \boldsymbol{\theta}_m}\Big) + o_p(1).$$

Moreover, by using the fact that $\rho(\mathbb{B}_0) < 1$, Lemma C.6 and the similar arguments as for Lemma A.11, we can show

$$\mathbf{U}_5 = \frac{1}{\sqrt{T}} \sum_{t=q+1}^{T} \text{vec}\Big(\frac{\partial \mathbf{g}_t}{\partial \boldsymbol{\theta}_m}\Big)' (\mathbf{g}_t^{-1})^{\otimes 2}$$

$$\times \sum_{k=0}^{\infty} \mathbb{B}_0^k(1:N^2, 1:N^2)\Big(\sum_{i=1}^{q} \mathcal{A}_{i0}\Big)[\boldsymbol{\tau}_t^{-3/4} \otimes \mathbf{u}_{t-k-i}\mathbf{u}_{t-k-i}'\boldsymbol{\tau}_t^{-1/4}]\text{vec}(\boldsymbol{\tau}_t - \widehat{\boldsymbol{\tau}}_t) + o_p(1).$$

Recall $\mathbf{M}_m = E\Big[\text{vec}\Big(\frac{\partial \mathbf{g}_t}{\partial \boldsymbol{\theta}_m}\Big)' (\mathbf{g}_t^{-1})^{\otimes 2}\mathbf{T}_t\Big]$ and $\mathbf{T}_t = \sum_{k=0}^{\infty} \mathbb{B}_0^k(1:N^2, 1:N^2)(\sum_{i=1}^{q} \mathcal{A}_{i0})[I_N \otimes \mathbf{u}_{t-k-i}\mathbf{u}_{t-k-i}']$. Then, by Lemma C.1 we have

$$\mathbf{U}_5 = \frac{1}{\sqrt{T}} \sum_{t=q+1}^{T} \text{vec}\Big(\frac{\partial \mathbf{g}_t}{\partial \boldsymbol{\theta}_m}\Big)' (\mathbf{g}_t^{-1})^{\otimes 2}\mathbf{T}_t \text{vec}\Big(\boldsymbol{\tau}_t^{-1/4}(\boldsymbol{\tau}_t - \widehat{\boldsymbol{\tau}}_t)\boldsymbol{\tau}_t^{-3/4}\Big) + o_p(1)$$

$$= -\frac{1}{\sqrt{T}} \sum_{t=q+1}^{T} \text{vec}\Big(\frac{\partial \mathbf{g}_t}{\partial \boldsymbol{\theta}_m}\Big)' (\mathbf{g}_t^{-1})^{\otimes 2}\mathbf{T}_t \text{vec}\Big(\frac{1}{T}\sum_{s=1}^{T} K_h\Big(\frac{t-s}{Th}\Big)\boldsymbol{\tau}_t^{1/4}(\mathbf{u}_s\mathbf{u}_s' - I_N)\boldsymbol{\tau}_t^{-1/4}\Big) + o_p(1)$$

$$= -\frac{1}{\sqrt{T}} \sum_{t=q+1}^{T} \text{vec}\Big(\frac{\partial \mathbf{g}_t}{\partial \boldsymbol{\theta}_m}\Big)' (\mathbf{g}_t^{-1})^{\otimes 2}\mathbf{T}_t[\boldsymbol{\tau}_t^{-1/4} \otimes \boldsymbol{\tau}_t^{1/4}]\frac{1}{T}\sum_{s=1}^{T} K_h\Big(\frac{t-s}{Th}\Big)\text{vec}(\mathbf{u}_s\mathbf{u}_s' - I_N) + o_p(1)$$

$$= -\frac{1}{\sqrt{T}} \sum_{t=q+1}^{T} \mathbf{M}_m[\boldsymbol{\tau}_t^{-1/4} \otimes \boldsymbol{\tau}_t^{1/4}]\frac{1}{T}\sum_{s=1}^{T} K_h\Big(\frac{t-s}{Th}\Big)\text{vec}(\mathbf{u}_s\mathbf{u}_s' - I_N) + o_p(1)$$

$$-\frac{1}{\sqrt{T}} \sum_{t=q+1}^{T} \Big\{\text{vec}\Big(\frac{\partial \mathbf{g}_t}{\partial \boldsymbol{\theta}_m}\Big)' [\mathbf{g}_t^{-1} \otimes \mathbf{g}_t^{-1}]\mathbf{T}_t - \mathbf{M}_m\Big\}$$

$$\times [\boldsymbol{\tau}_t^{-1/4} \otimes \boldsymbol{\tau}_t^{1/4}]\frac{1}{T}\sum_{s=1}^{T} K_h\Big(\frac{t-s}{Th}\Big)\text{vec}(\mathbf{u}_s\mathbf{u}_s' - I_N) + o_p(1) =: \mathbf{U}_{51}^* + \mathbf{U}_{52}^* + o_p(1).$$

By Proposition A.1, we can obtain that $\mathbf{U}_{52}^* = o_p(1)$. Hence, by using the fact that $\boldsymbol{\tau}_s^{-1/4} = \boldsymbol{\tau}_t^{-1/4} + o(1)$ for $|t-s| < Th$, we have

$$\mathbf{U}_5 = \mathbf{U}_{51}^* + o_p(1) = -\frac{1}{\sqrt{T}} \sum_{s=1}^{T} \mathbf{M}_m[\boldsymbol{\tau}_s^{-1/4} \otimes \boldsymbol{\tau}_s^{1/4}]\text{vec}(\mathbf{u}_s\mathbf{u}_s' - I_N) + o_p(1).$$

This completes the proof. □

Lemma C.9. *Under the conditions in Theorem 6.1,* $U_9 = \frac{1}{\sqrt{T}}\sum_{t=1}^{T} \mathbf{N}_m[\boldsymbol{\tau}_t^{-1/4} \otimes \boldsymbol{\tau}_t^{1/4}]\text{vec}(\mathbf{u}_t\mathbf{u}_t' - I_N) + o_p(1)$.

Proof of Lemma C.9. By Lemmas C.4 and C.2(i), we can show

$$\mathbf{U}_9 = -\frac{1}{\sqrt{T}} \sum_{t=1}^{T} \text{vec}\Big(\frac{\partial \mathbf{g}_t}{\partial \boldsymbol{\theta}_m}\Big)' (\mathbf{g}_t^{-1})^{\otimes 2}\Delta_t + o_p(1)$$

$$= -\frac{1}{\sqrt{T}}\sum_{t=1}^{T}\mathrm{vec}\Big(\frac{\partial \mathbf{g}_t}{\partial \boldsymbol{\theta}_m}\Big)'(\mathbf{g}_t^{-1})^{\otimes 2}\frac{1}{2}\Big([\boldsymbol{\tau}_t^{-3/4}\otimes \mathbf{u}_t\mathbf{u}_t'\boldsymbol{\tau}_t^{-1/4}] + [\mathbf{u}_t\mathbf{u}_t'\boldsymbol{\tau}_t^{-1/4}\otimes \boldsymbol{\tau}_t^{-3/4}]\Big)\mathrm{vec}(\boldsymbol{\tau}_t - \widehat{\boldsymbol{\tau}}_t)$$
$$+ o_p(1)$$
$$= -\frac{1}{\sqrt{T}}\sum_{t=1}^{T}\mathrm{tr}\Big(\frac{\partial \mathbf{g}_t}{\partial \boldsymbol{\theta}_m}\mathbf{g}_t^{-1}\mathbf{u}_t\mathbf{u}_t'\boldsymbol{\tau}^{-1/4}(\boldsymbol{\tau}_t - \widehat{\boldsymbol{\tau}}_t)\boldsymbol{\tau}^{-3/4}\mathbf{g}_t^{-1}\Big) + o_p(1)$$
$$= -\frac{1}{\sqrt{T}}\sum_{t=1}^{T}\mathrm{tr}\Big(\frac{\partial \mathbf{g}_t}{\partial \boldsymbol{\theta}_m}\mathbf{g}_t^{-1/2}\boldsymbol{\eta}_t\boldsymbol{\eta}_t'\mathbf{g}_t^{1/2}\boldsymbol{\tau}^{-1/4}(\boldsymbol{\tau}_t - \widehat{\boldsymbol{\tau}}_t)\boldsymbol{\tau}^{-3/4}\mathbf{g}_t^{-1}\Big) + o_p(1).$$

Then, by Lemma C.1, we can obtain

$$\mathbf{U}_9 = \frac{1}{\sqrt{T}}\sum_{t=1}^{T}\mathrm{vec}(\frac{\partial \mathbf{g}_t}{\partial \boldsymbol{\theta}_m})'[\mathbf{g}_t^{-1}\otimes \mathbf{g}_t^{-1/2}\boldsymbol{\eta}_t\boldsymbol{\eta}_t'\mathbf{g}_t^{1/2}][\boldsymbol{\tau}_t^{-1/4}\otimes \boldsymbol{\tau}_t^{1/4}]$$
$$\times \frac{1}{T}\sum_{s=1}^{T}K_h\Big(\frac{t-s}{Th}\Big)\mathrm{vec}(\mathbf{u}_s\mathbf{u}_s' - I_N) + o_p(1).$$

By the similar arguments as in Proposition A.1, it follows that

$$\mathbf{U}_9 = \frac{1}{\sqrt{T}}\sum_{t=1}^{T}\mathbf{N}_m[\boldsymbol{\tau}_t^{-1/4}\otimes \boldsymbol{\tau}_t^{1/4}]\frac{1}{T}\sum_{s=1}^{T}K_h\Big(\frac{t-s}{Th}\Big)\mathrm{vec}(\mathbf{u}_s\mathbf{u}_s' - I_N) + o_p(1).$$

Now, the result follows by using the fact that $\boldsymbol{\tau}_s^{-1/4} = \boldsymbol{\tau}_t^{-1/4} + o(1)$ for $|t-s| < Th$. □

Proof of Theorem 6.1. By Taylor's expansion, it follows that

$$\sqrt{T}(\widehat{\boldsymbol{\theta}}_T - \boldsymbol{\theta}_0) = -\Big[\frac{1}{T}\sum_{t=1}^{T}\frac{\partial^2 \widehat{\mathbf{l}}_t(\boldsymbol{\theta}^*)}{\partial \boldsymbol{\theta}\partial \boldsymbol{\theta}'}\Big]^{-1}\frac{1}{\sqrt{T}}\frac{\partial \widehat{\mathbf{L}}_t(\boldsymbol{\theta}_0)}{\partial \boldsymbol{\theta}},$$

where $\boldsymbol{\theta}^*$ lies between $\boldsymbol{\theta}_0$ and $\widehat{\boldsymbol{\theta}}_T$.

By Lemmas C.1–C.4, it is not hard to see that $\mathbf{U}_i = o_p(1)$ for $i = 4, 6, 7, 8, 10, 11, 12$, and

$$\mathbf{U}_1 = \frac{1}{\sqrt{T}}\frac{\partial \mathbf{L}_t(\boldsymbol{\theta}_0)}{\partial \boldsymbol{\theta}_m} + o_p(1) = -\frac{1}{\sqrt{T}}\sum_{t=1}^{T}\mathbf{Q}_{t,m}\boldsymbol{\xi}_t + o_p(1).$$

Hence, by Lemmas C.7–C.9 and (C.3), we have

$$\frac{1}{\sqrt{T}}\frac{\partial \widehat{\mathbf{L}}_T(\boldsymbol{\theta}_0)}{\partial \boldsymbol{\theta}_m} = -\frac{1}{\sqrt{T}}\sum_{t=1}^{T}\mathbf{Q}_{t,m}\boldsymbol{\xi}_t - \frac{1}{\sqrt{T}}\sum_{t=1}^{T}[\mathbf{M}_m - \mathbf{N}_m][\boldsymbol{\tau}_t^{-1/4}\otimes \boldsymbol{\tau}_t^{1/4}]\mathbf{z}_t + o_p(1),$$

where $\mathbf{z}_t = \mathrm{vec}(\mathbf{u}_t\mathbf{u}_t' - I_N)$.

Next, we calculate the asymptotic variance-covariance matrix of $\frac{1}{\sqrt{T}}\frac{\partial \widehat{\mathbf{L}}_T(\boldsymbol{\theta}_0)}{\partial \boldsymbol{\theta}}$, i.e.,

$$\lim_{T\to\infty}\mathrm{Var}\Big(\frac{1}{\sqrt{T}}\frac{\partial \widehat{\mathbf{L}}_T(\boldsymbol{\theta}_0)}{\partial \boldsymbol{\theta}}\Big)$$

$$
\begin{aligned}
&= \lim_{T\to\infty} \mathrm{Var}\Big(\frac{1}{\sqrt{T}}\sum_{t=1}^{T}\mathbf{Q}_t\xi_t\Big) + \lim_{T\to\infty} \mathrm{Var}\Big(\frac{1}{\sqrt{T}}\sum_{t=1}^{T}[\mathbf{M}-\mathbf{N}][\boldsymbol{\tau}_t^{-1/4}\otimes\boldsymbol{\tau}_t^{1/4}]\mathbf{z}_t\Big)\\
&\quad + \lim_{T\to\infty} \mathrm{Cov}\Big(\frac{1}{\sqrt{T}}\sum_{t=1}^{T}\mathbf{Q}_t\xi_t, \frac{1}{\sqrt{T}}\sum_{t=1}^{T}[\mathbf{M}-\mathbf{N}][\boldsymbol{\tau}_t^{-1/4}\otimes\boldsymbol{\tau}_t^{1/4}]\mathbf{z}_t\Big)\\
&\quad + \lim_{T\to\infty} \mathrm{Cov}\Big(\frac{1}{\sqrt{T}}\sum_{t=1}^{T}\mathbf{Q}_t\xi_t, \frac{1}{\sqrt{T}}\sum_{t=1}^{T}[\mathbf{M}-\mathbf{N}][\boldsymbol{\tau}_t^{-1/4}\otimes\boldsymbol{\tau}_t^{1/4}]\mathbf{z}_t\Big)'\\
&=: \mathbf{J}_1 + \mathbf{J}_2 + \mathbf{J}_3 + \mathbf{J}_3'.
\end{aligned}
$$

Clearly, $\mathbf{J}_1 = E\Big[\mathbf{Q}_t\mathrm{Var}(\boldsymbol{\xi}_t)\mathbf{Q}_t'\Big]$. By some direct calculation, we have

$$
\begin{aligned}
\mathbf{J}_2 &= \lim_{T\to\infty} \mathrm{Var}\Big(\frac{1}{\sqrt{T}}\sum_{t=1}^{T}[\mathbf{M}-\mathbf{N}][\boldsymbol{\tau}_t^{-1/4}\otimes\boldsymbol{\tau}_t^{1/4}]\mathbf{z}_t\Big)\\
&= [\mathbf{M}-\mathbf{N}]\int_0^1 \boldsymbol{\Upsilon}(x)\sum_{j=-\infty}^{\infty} E[\mathbf{z}_t\mathbf{z}_{t-j}']\boldsymbol{\Upsilon}(x)[\mathbf{M}-\mathbf{N}]'dx.
\end{aligned}
$$

Moreover, by Lemma C.10 below, we have

$$
\sum_{j=-\infty}^{\infty} E[\mathbf{z}_t\mathbf{z}_{t-j}'] = \lim_{T\to\infty}\mathrm{Var}\Big(\frac{1}{\sqrt{T}}\sum_{t=1}^{T}\mathbf{z}_t\Big) = \boldsymbol{\Omega}_0^{-1}\boldsymbol{\Gamma}_0 E\Big[(\mathbf{g}_t^{1/2})^{\otimes 2}\mathrm{Var}(\boldsymbol{\xi}_t)(\mathbf{g}_t^{1/2})^{\otimes 2}\Big]\boldsymbol{\Gamma}_0'\boldsymbol{\Omega}_0'^{-1},
$$

and hence,

$$
\mathbf{J}_2 = [\mathbf{M}-\mathbf{N}]\Big\{\int_0^1 \boldsymbol{\Upsilon}(x)\boldsymbol{\Omega}_0^{-1}\boldsymbol{\Gamma}_0 E\Big[(\mathbf{g}_t^{1/2})^{\otimes 2}\mathrm{Var}(\boldsymbol{\xi}_t)(\mathbf{g}_t^{1/2})^{\otimes 2}\Big]\boldsymbol{\Gamma}_0'\boldsymbol{\Omega}_0'^{-1}\boldsymbol{\Upsilon}(x)dx\Big\}[\mathbf{M}-\mathbf{N}]'.
$$

Similarly, we can show

$$
\begin{aligned}
\mathbf{J}_3 &= \lim_{T\to\infty}\mathrm{Cov}\Big(\frac{1}{\sqrt{T}}\sum_{t=1}^{T}\mathbf{Q}_t\boldsymbol{\xi}_t, \frac{1}{\sqrt{T}}\sum_{t=1}^{T}[\mathbf{M}-\mathbf{N}][\boldsymbol{\tau}_t^{-1/4}\otimes\boldsymbol{\tau}_t^{1/4}]\mathbf{z}_t\Big)\\
&= \sum_{j=-\infty}^{\infty} E\Big[\mathbf{Q}_t\boldsymbol{\xi}_t\mathbf{z}_{t-j}'\Big]\int_0^1 \boldsymbol{\Upsilon}(x)dx[\mathbf{M}-\mathbf{N}]',
\end{aligned}
$$

where by using Lemma C.10 again,

$$
\begin{aligned}
\sum_{j=-\infty}^{\infty} E\Big[\mathbf{Q}_t\boldsymbol{\xi}_t\mathbf{z}_{t-j}'\Big] &= \lim_{T\to\infty}\mathrm{Cov}\Big(\frac{1}{\sqrt{T}}\sum_{t=1}^{T}\mathbf{Q}_t\boldsymbol{\xi}_t, \frac{1}{\sqrt{T}}\sum_{t=1}^{T}\mathbf{z}_t\Big)\\
&= E\Big[\mathbf{Q}_t\mathrm{Var}(\boldsymbol{\xi}_t)(\mathbf{g}_t^{1/2})^{\otimes 2}\Big]\boldsymbol{\Gamma}_0'\boldsymbol{\Omega}_0'^{-1}.
\end{aligned}
$$

Hence,

$$
\mathbf{J}_3 = E\Big[\mathbf{Q}_t\mathrm{Var}(\boldsymbol{\xi}_t)(\mathbf{g}_t^{1/2})^{\otimes 2}\Big]\Big\{\boldsymbol{\Gamma}_0'\boldsymbol{\Omega}_0'^{-1}\int_0^1 \boldsymbol{\Upsilon}(x)dx\Big\}[\mathbf{M}-\mathbf{N}]'.
$$

So, by the martingale central limit theorem, we have

$$
\frac{1}{\sqrt{T}}\frac{\partial\widehat{\mathbf{L}}_t(\boldsymbol{\theta}_0)}{\partial\boldsymbol{\theta}} \to_{\mathcal{L}} N(0, \mathbf{J}_1 + \mathbf{J}_2 + \mathbf{J}_3 + \mathbf{J}_3') \text{ as } T\to\infty.
$$

Finally, we consider $\frac{1}{T}\sum_{t=1}^{T}\frac{\partial^2\widehat{\mathbf{l}}_t(\boldsymbol{\theta}^*)}{\partial\boldsymbol{\theta}\partial\boldsymbol{\theta}'}$. Due to the consistency of $\widehat{\boldsymbol{\theta}}_T$, we can show

$$\frac{1}{T}\sum_{t=1}^{T}\frac{\partial^2\widehat{\mathbf{l}}_t(\boldsymbol{\theta}^*)}{\partial\boldsymbol{\theta}\partial\boldsymbol{\theta}'}\rightarrow_p E\Big[\frac{\partial^2\mathbf{l}_t(\boldsymbol{\theta}_0)}{\partial\boldsymbol{\theta}\partial\boldsymbol{\theta}'}\Big].$$

We now calculate $E\Big[\frac{\partial^2\mathbf{l}_t(\boldsymbol{\theta}_0)}{\partial\boldsymbol{\theta}\partial\boldsymbol{\theta}'}\Big]$. For any $1\le i,j\le\dim(\boldsymbol{\theta})$, we have

$$\begin{aligned}\frac{\partial^2\mathbf{l}_t(\boldsymbol{\theta}_0)}{\partial\boldsymbol{\theta}_i\partial\boldsymbol{\theta}_j}=&\mathrm{tr}\Big(\mathbf{g}_t^{-1}\frac{\partial^2\mathbf{g}_t}{\partial\boldsymbol{\theta}_i\partial\boldsymbol{\theta}_j}\Big)-\mathrm{tr}\Big(\mathbf{g}_t^{-1}\frac{\partial\mathbf{g}_t}{\partial\boldsymbol{\theta}_i}\mathbf{g}_t^{-1}\frac{\partial\mathbf{g}_t}{\partial\boldsymbol{\theta}_j}\Big)\\&+2\mathrm{tr}\Big(\mathbf{g}_t^{-1}\mathbf{u}_t\mathbf{u}_t'\mathbf{g}_t^{-1}\frac{\partial\mathbf{g}_t}{\partial\boldsymbol{\theta}_i}\mathbf{g}_t^{-1}\frac{\partial\mathbf{g}_t}{\partial\boldsymbol{\theta}_j}\Big)-\mathrm{tr}\Big(\mathbf{g}_t^{-1}\mathbf{u}_t\mathbf{u}_t'\mathbf{g}_t^{-1}\frac{\partial^2\mathbf{g}_t}{\partial\boldsymbol{\theta}_i\partial\boldsymbol{\theta}_j}\Big).\end{aligned}$$

Hence,

$$E\frac{\partial^2\mathbf{l}_t(\boldsymbol{\theta}_0)}{\partial\boldsymbol{\theta}_i\partial\boldsymbol{\theta}_j}=E\mathrm{tr}\Big(\mathbf{g}_t^{-1}\frac{\partial\mathbf{g}_t}{\partial\boldsymbol{\theta}_i}\mathbf{g}_t^{-1}\frac{\partial\mathbf{g}_t}{\partial\boldsymbol{\theta}_j}\Big),$$

which entails that $E\Big[\frac{\partial^2\mathbf{l}_t(\boldsymbol{\theta}_0)}{\partial\boldsymbol{\theta}\partial\boldsymbol{\theta}'}\Big]=E[\mathbf{Q}_t\mathbf{Q}_t']$. This completes the proof. □

LEMMA C.10. *Under the conditions in Theorem 6.1,*

$$\frac{1}{\sqrt{T}}\sum_{t=1}^{T}\mathbf{z}_t=\boldsymbol{\Omega}_0^{-1}\boldsymbol{\Gamma}_0\frac{1}{\sqrt{T}}\sum_{t=1}^{T}(\mathbf{g}_t^{1/2})^{\otimes 2}\boldsymbol{\xi}_t+o_p(1).$$

PROOF OF LEMMA C.10. Since $\mathbf{u}_t\mathbf{u}_t'-I_N=\mathbf{g}_t^{1/2}(\boldsymbol{\eta}_t\boldsymbol{\eta}_t'-I_N)\mathbf{g}_t^{1/2}+\mathbf{g}_t-I_N$, we have

$$\begin{aligned}&\mathbf{u}_t\mathbf{u}_t'-I_N\\=&\mathbf{g}_t^{1/2}(\boldsymbol{\eta}_t\boldsymbol{\eta}_t'-I_N)\mathbf{g}_t^{1/2}+\sum_{i=1}^{q}A_{i0}(\mathbf{u}_{t-i}\mathbf{u}_{t-i}'-I_N)A_{i0}'+\sum_{j=1}^{p}B_{j0}(\mathbf{g}_{t-j}-I_N)B_{j0}'\\=&\mathbf{g}_t^{1/2}(\boldsymbol{\eta}_t\boldsymbol{\eta}_t'-I_N)\mathbf{g}_t^{1/2}+\sum_{i=1}^{q}A_{i0}(\mathbf{u}_{t-i}\mathbf{u}_{t-i}'-I_N)A_{i0}'+\sum_{j=1}^{p}B_{j0}(\mathbf{u}_{t-j}\mathbf{u}_{t-j}'-I_N)B_{j0}'\\&-\sum_{j=1}^{p}B_{j0}\mathbf{g}_{t-j}^{1/2}(\boldsymbol{\eta}_{t-j}\boldsymbol{\eta}_{t-j}'-I_N)\mathbf{g}_{t-j}^{1/2}B_{j0}'.\end{aligned}$$

Hence, we can obtain

$$\begin{aligned}\frac{1}{\sqrt{T}}\sum_{t=1}^{T}\mathbf{z}_t=&\frac{1}{\sqrt{T}}\sum_{t=1}^{T}(\mathbf{g}_t^{1/2})^{\otimes 2}\boldsymbol{\xi}_t+\frac{1}{\sqrt{T}}\sum_{t=1}^{T}\sum_{i=1}^{q}\mathcal{A}_{i0}\mathbf{z}_{t-i}+\frac{1}{\sqrt{T}}\sum_{t=1}^{T}\sum_{j=1}^{p}\mathcal{B}_{j0}\mathbf{z}_{t-j}\\&-\frac{1}{\sqrt{T}}\sum_{t=1}^{T}\sum_{j=1}^{p}\mathcal{B}_{j0}(\mathbf{g}_{t-j}^{1/2})^{\otimes 2}\boldsymbol{\xi}_{t-j}.\end{aligned}$$

By the similar arguments as for (A.8) with the convention $\mathcal{B}_{j0}=0$ if $j>p$ and $\mathcal{A}_{i0}=0$ if $i>q$, we have

$$\frac{1}{\sqrt{T}}\sum_{t=1}^{T}\mathbf{z}_t=\frac{1}{\sqrt{T}}\sum_{t=1}^{T}\sum_{i=1}^{\max\{p,q\}}[\mathcal{A}_{i0}+\mathcal{B}_{i0}]\mathbf{z}_{t-i}+\frac{1}{\sqrt{T}}\sum_{t=1}^{T}(\mathbf{g}_t^{1/2})^{\otimes 2}\boldsymbol{\xi}_t$$

$$-\frac{1}{\sqrt{T}}\sum_{t=1}^{T}\sum_{j=1}^{p}\mathcal{B}_{j0}(\mathbf{g}_{t-j}^{1/2})^{\otimes 2}\boldsymbol{\xi}_{t-j}.$$

Hence, it follows that

$$\frac{1}{\sqrt{T}}\sum_{t=1}^{T}\mathbf{z}_t=\Big[I_{N^2}-\sum_{i=1}^{q}\mathcal{A}_{i0}-\sum_{j=1}^{p}\mathcal{B}_{j0}\Big]^{-1}\Big[I_{N^2}-\sum_{j=1}^{p}\mathcal{B}_{j0}\Big]\frac{1}{\sqrt{T}}\sum_{t=1}^{T}(\mathbf{g}_t^{1/2})^{\otimes 2}\boldsymbol{\xi}_t+o_p(1).$$

This completes the proof. □.

## REFERENCES


[1] Amemiya, T., 1985. *Advanced Econometrics.* Harvard University Press.

[2] Carrasco, M., Chen, X., 2002. Mixing and moment properties of various GARCH and stochastic volatility Models. *Econometric Theory* **18**, 17–39.

[3] Francq, C., Zakoïan, J.M., 2004. Maximum likelihood estimation of pure GARCH and ARMA-GARCH processes. *Bernoulli* **10**, 605–637.

[4] Francq, C., Zakoïan, J.M., 2010. QML estimation of a class of multivariate asymmetric GARCH models. *Econometric Theory* **28**, 179–206.

[5] Hall, P., Heyde, C.C., 1980. *Martingale Limit Theory and its Applications.* Academic Press.

[6] Hafner, C.M. Linton, O., 2010. Efficient estimation of a multivariate multiplicative volatility model. *Journal of Econometrics* **159**, 55–73.
